# Supplementary material for: Blind Visual Motif Removal from a Single Image
Source: arXiv:1904.02756 ancillary file (2019-04-04)
Supplement: Supplementary file 1 [file 2843-supp.pdf]

# Blind Visual Motif Removal from a Single Image

## Supplementary Material

Amir Hertz      Sharon Fogel      Rana Hanocka      Raja Giryes      Daniel Cohen-Or  
Tel Aviv University

This document contains some additional experiments to the paper “Blind Visual Motif Removal from a Single Image”. In Section 1 we show some additional visual examples of the removal of visual motifs with a comparison to other methods. Section 2 presents some additional inpainting experiments. In particular, we present our results on blind inpainting results demonstrated in other papers. Finally, Section 3 exhibits some additional ablation study experiments.

### 1. Transparent visual motifs removal results

Additional comparisons to [1, 2, 3, 4] for removal of a semi-transparent visual motif are shown in Figures 1 – 4.

In Figures 5 – 12 we show additional semi-transparent visual motif removal results on different types of motifs. To illustrate that the network can generalize to objects it hasn’t seen during training, we show in Figures 13 and 14 examples of motifs removed at test time and the 5 nearest Euclidean neighbours from the training set. In Figures 15 – 19 we show examples of watermark removal from various protected stock images using a single network, trained on our synthetic dataset.

### 2. Inpainting

In addition to the comparison presented in the paper, we used our pre-trained network on sample images from the previous methods’ papers. In Figure 20 we compare against the sample image from Shepard CNN [5]. In Figure 21 we compare to EPLL [6] and FoE [7] using their sample image.

### 3. Ablation study

Figure 22 shows a qualitative comparison between the different architectures in the ablation study. The network configurations we compared includes an auto-encoder U-Net model, baseline two-branch model, three-branch model with a separated branch for the motif (Baseline + Vm) and the chosen model (Baseline + shared Vm) with three branches as well as shared weight between the image and the motif decoders.

## References

- [1] Tali Dekel, Michael Rubinstein, Ce Liu, and William T Freeman. On the effectiveness of visible watermarks.
- [2] Anat Levin, Dani Lischinski, and Yair Weiss. A closed-form solution to natural image matting. *IEEE transactions on pattern analysis and machine intelligence*, 30(2):228–242, 2008.
- [3] Xuaner Zhang, Ren Ng, and Qifeng Chen. Single image reflection separation with perceptual losses. *CVPR*, 2018.
- [4] Jie Yang, Dong Gong, Lingqiao Liu, and Qinfeng Shi. Seeing deeply and bidirectionally: A deep learning approach for single image reflection removal. In *The European Conference on Computer Vision (ECCV)*, September 2018.
- [5] Jimmy SJ Ren, Li Xu, Qiong Yan, and Wenxiu Sun. Shepard convolutional neural networks. In *Advances in Neural Information Processing Systems*, pages 901–909, 2015.
- [6] Daniel Zoran and Yair Weiss. From learning models of natural image patches to whole image restoration. In *Computer Vision (ICCV), 2011 IEEE International Conference on*, pages 479–486. IEEE, 2011.
- [7] Stefan Roth and Michael J Black. Fields of experts. *International Journal of Computer Vision*, 82(2):205, 2009.

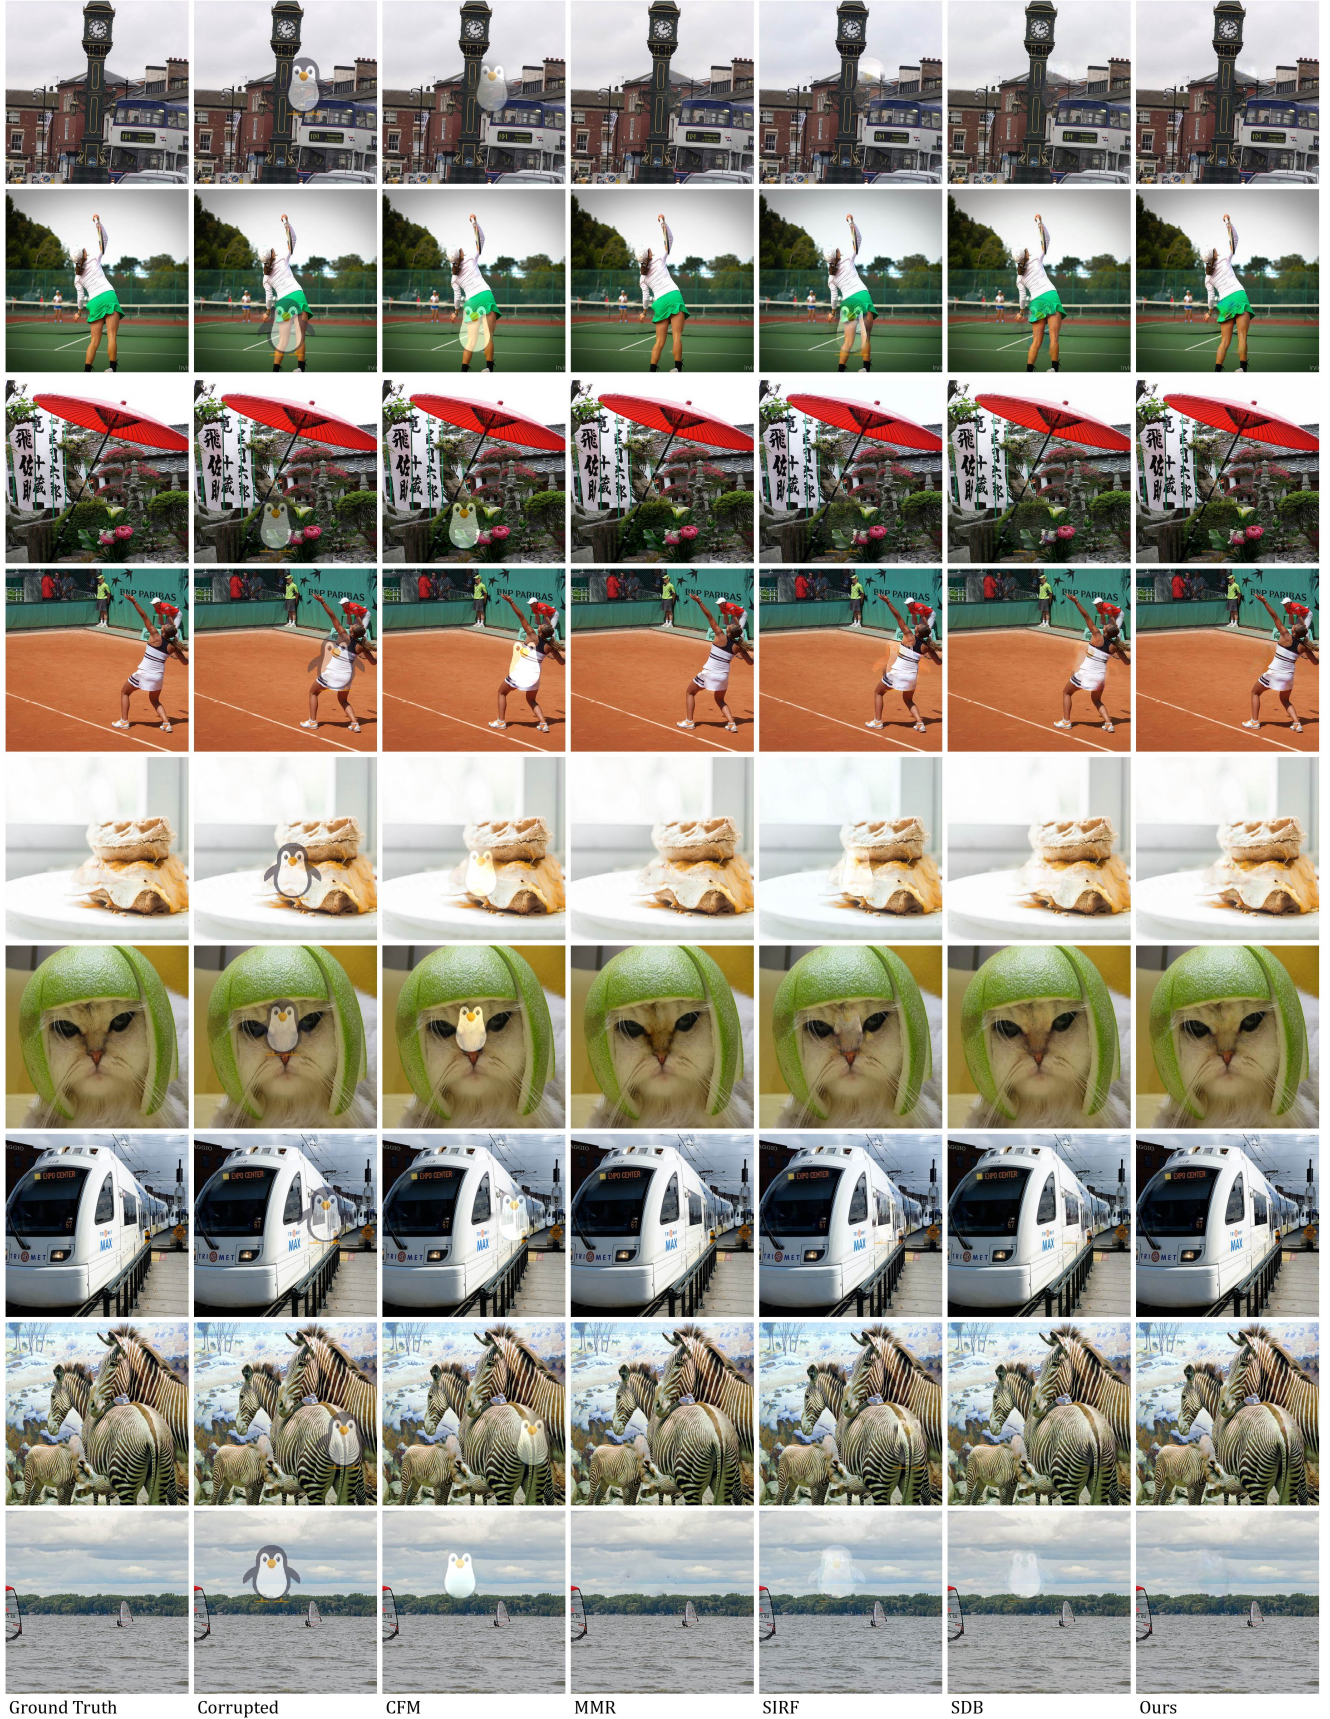

Figure 1: Visual comparisons to [1, 2, 3, 4] for removing a single transparent visual motif from multi image collection. Group A: We use a random translation and random constant opacity  $\alpha \in (0.4, 0.6)$  for blending the motif in each image.

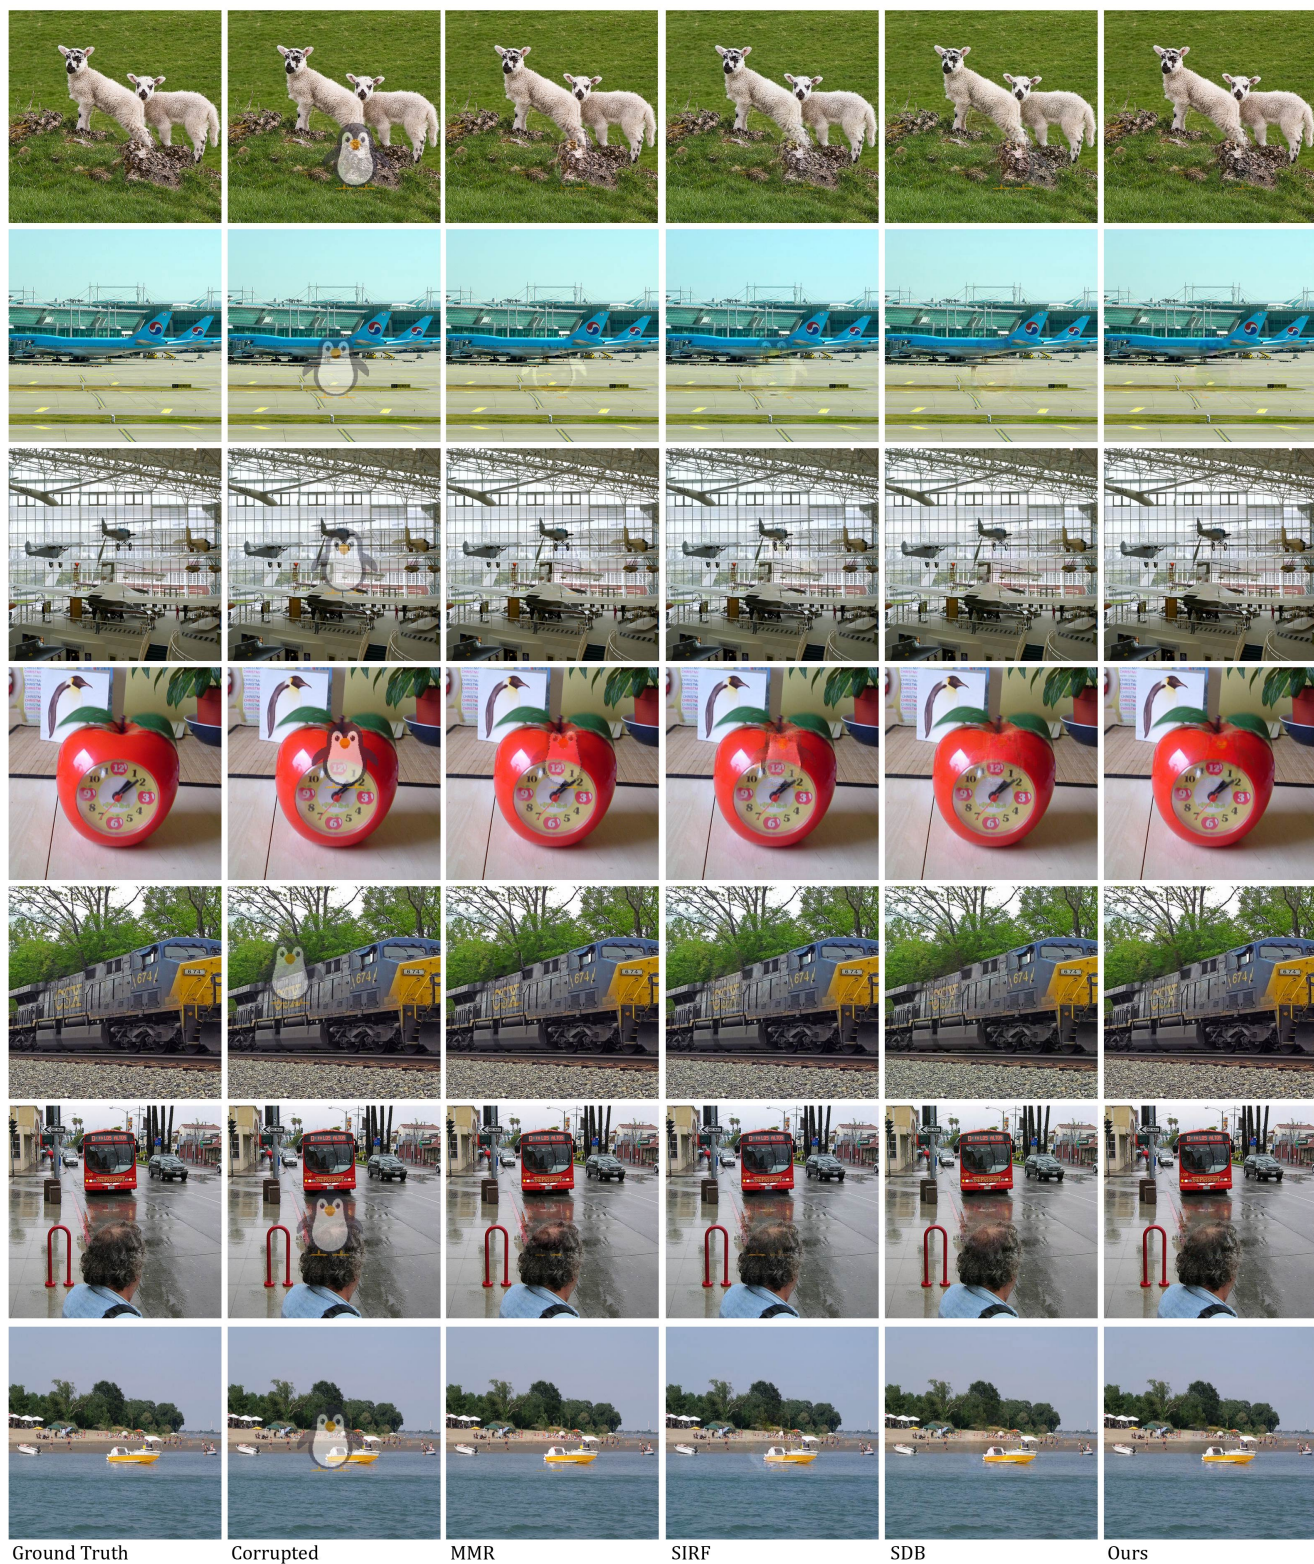

Figure 2: Visual comparisons to [1, 3, 4] for removing a single transparent visual motif from multi image collection. Group B: We add a random 1 pixel perturbations and varying opacity for the visual motif in each image.

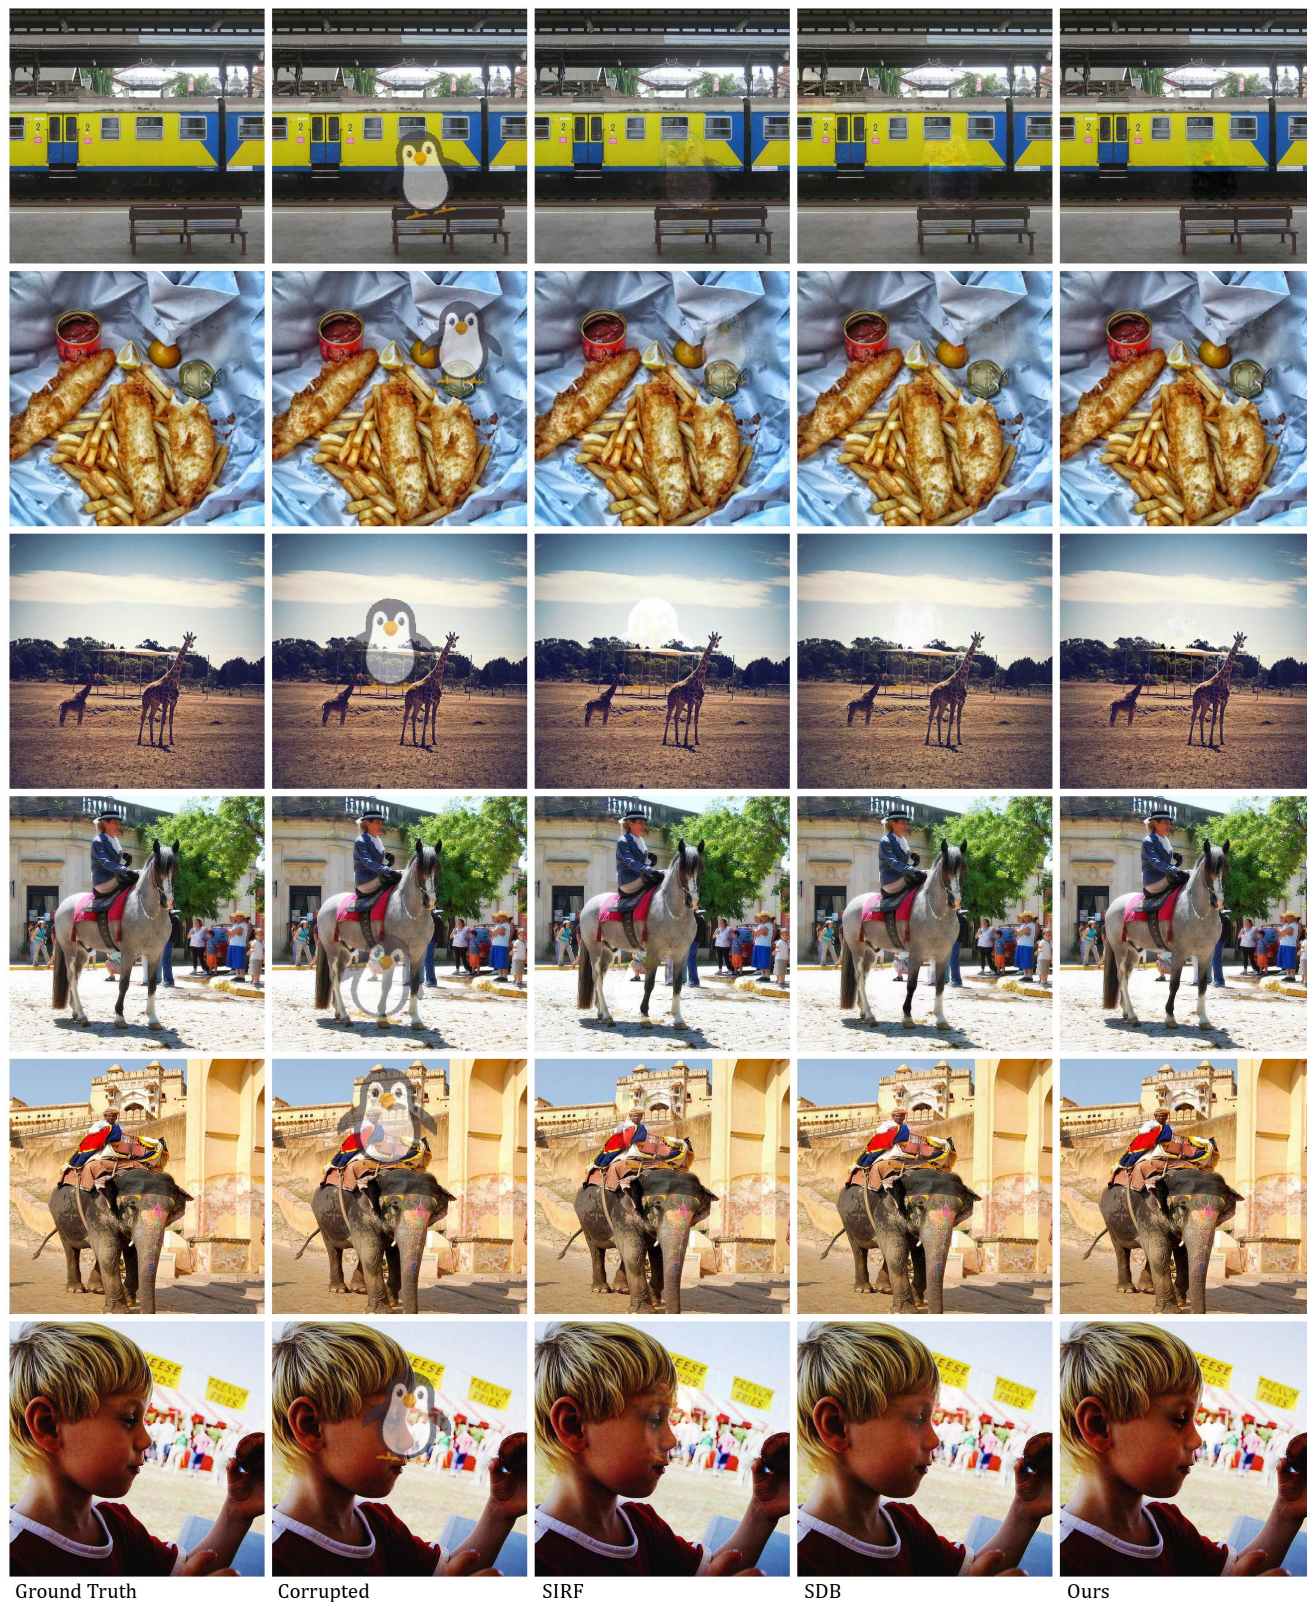

Figure 3: Visual comparisons to [3, 4] for removing a single transparent visual motif from a multi image collection. Group C: We add scale and rotation variations for the visual motif in each image.

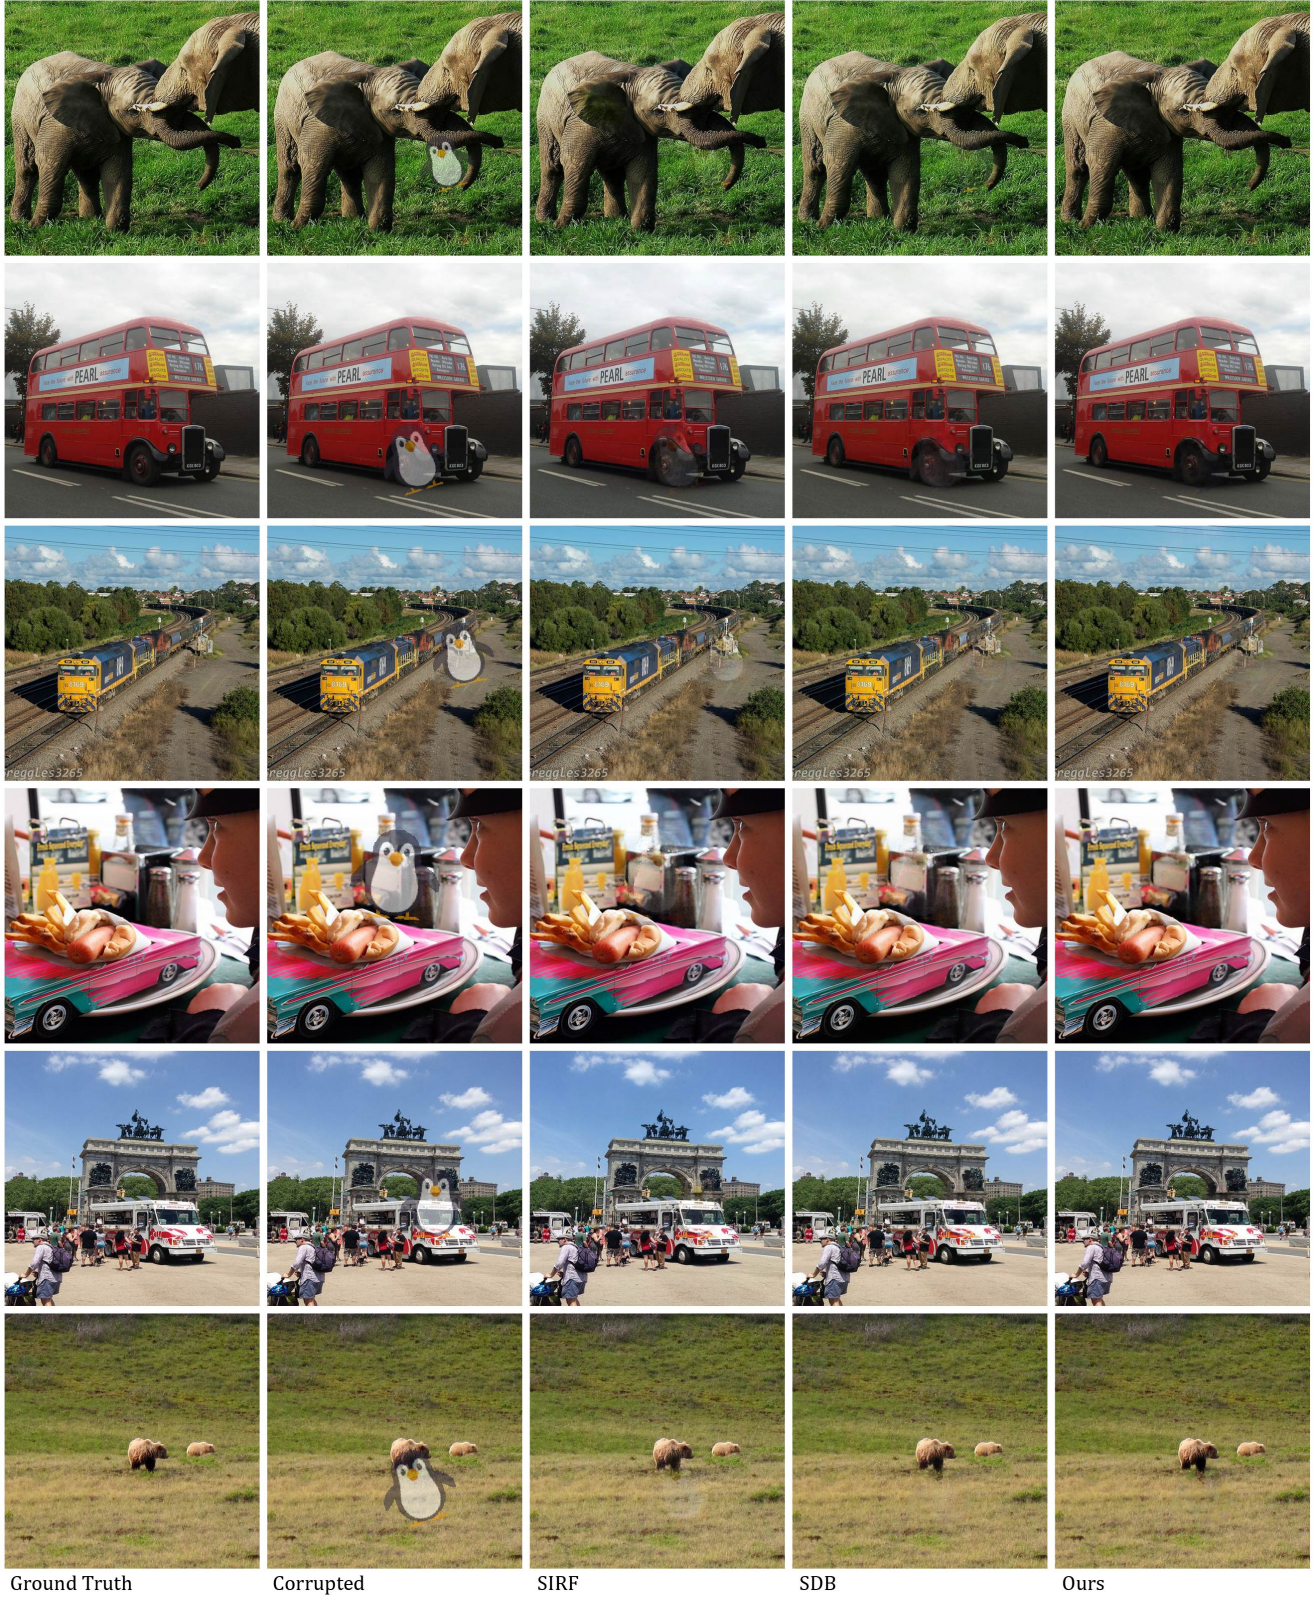

Figure 4: Visual comparisons to [3, 4] for removing a single transparent visual motif from a multi image collection. Group C: We add scale and rotation variations for the visual motif in each image.

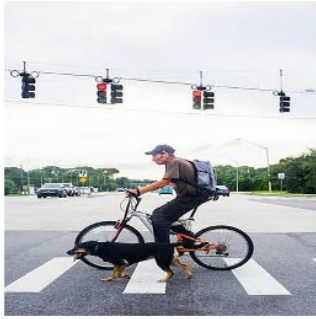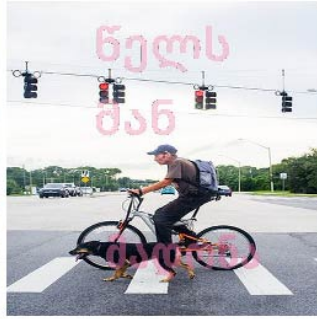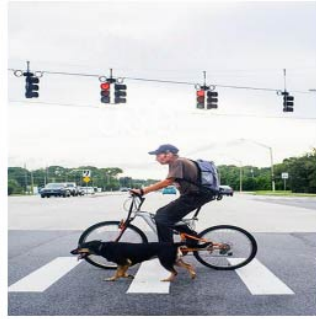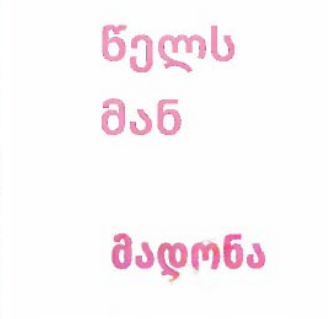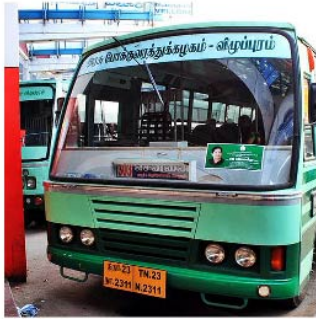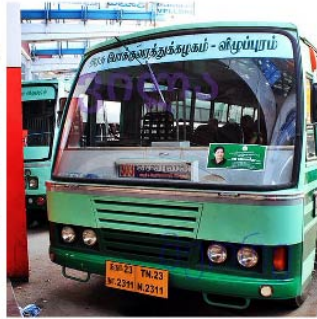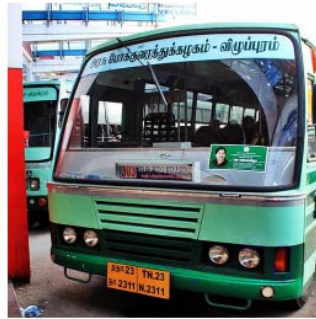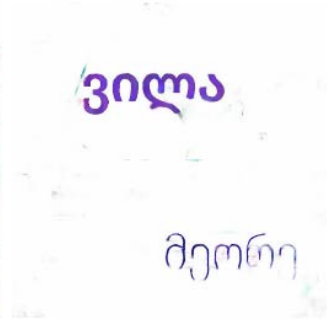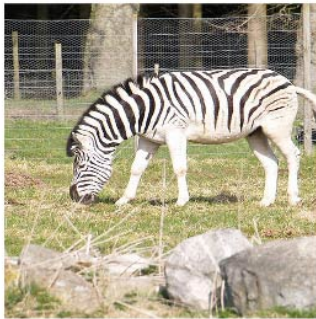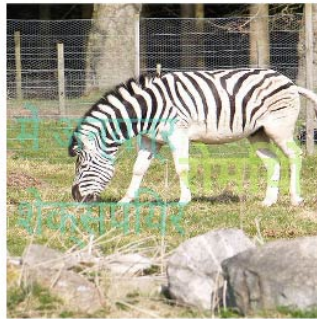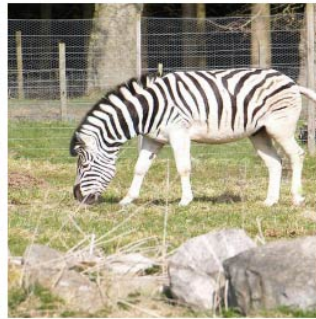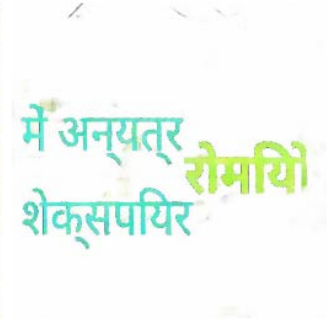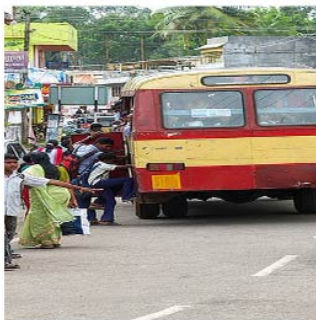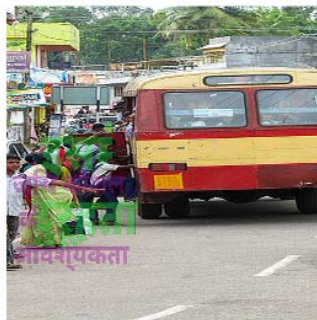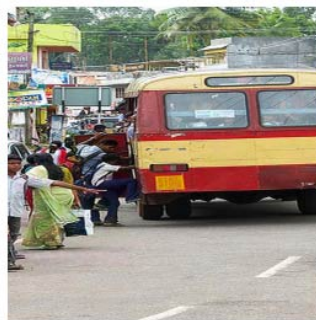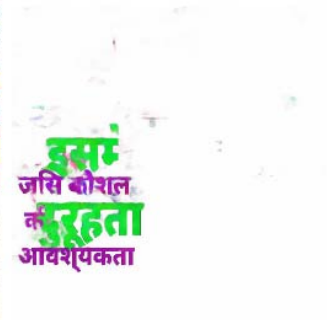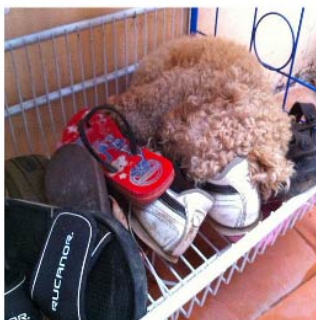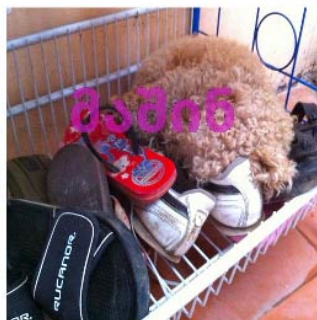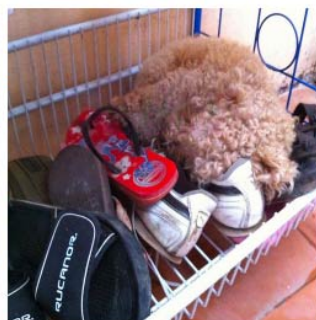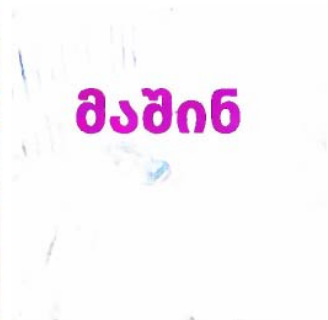

Ground Truth

Corrupted

Reconstructed Image

Reconstructed Motif

Figure 5: Examples of semi-transparent visual motif removal results. The test images contains unseen images and unseen characters as the visual motif.

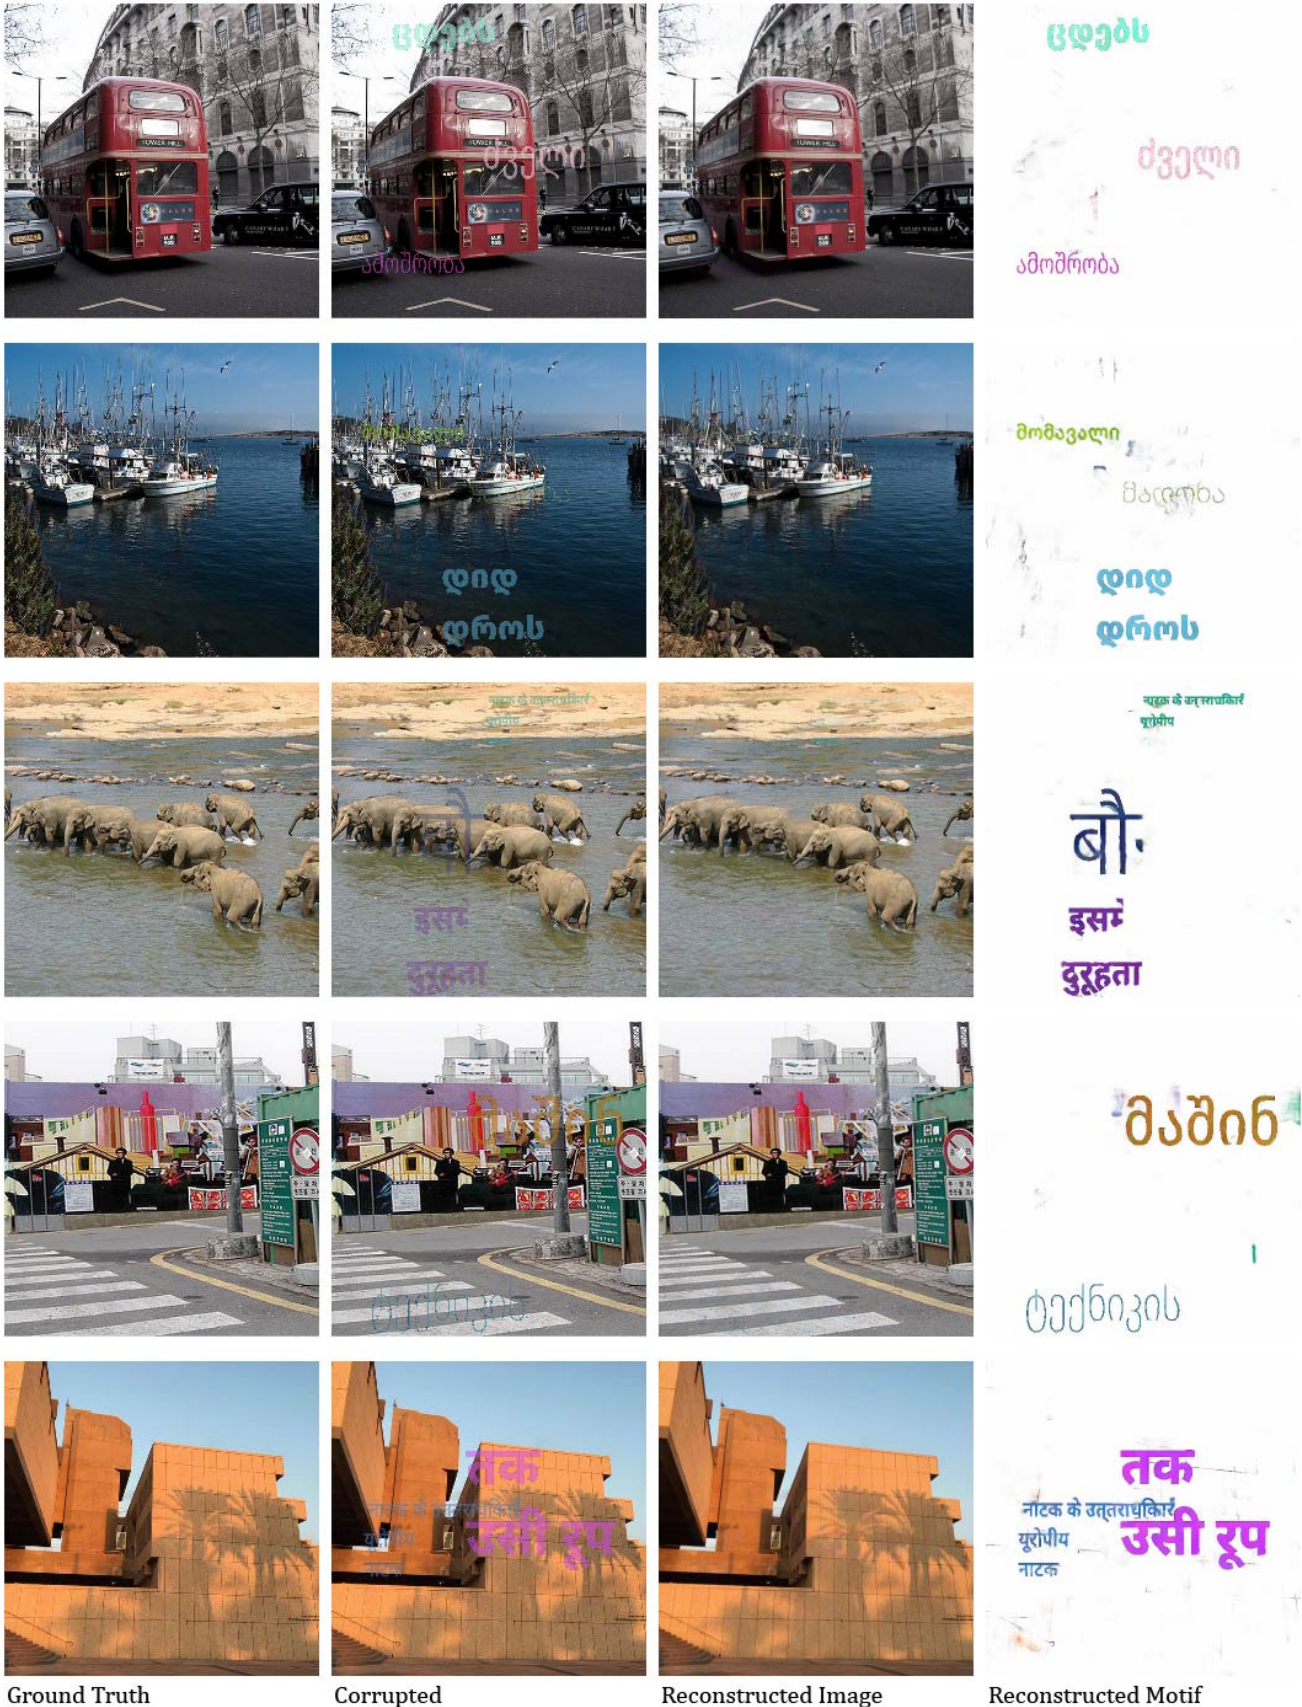

Ground Truth

Corrupted

Reconstructed Image

Reconstructed Motif

Figure 6: Examples of semi-transparent visual motif removal results. The test images contains unseen images and unseen characters as the visual motif.

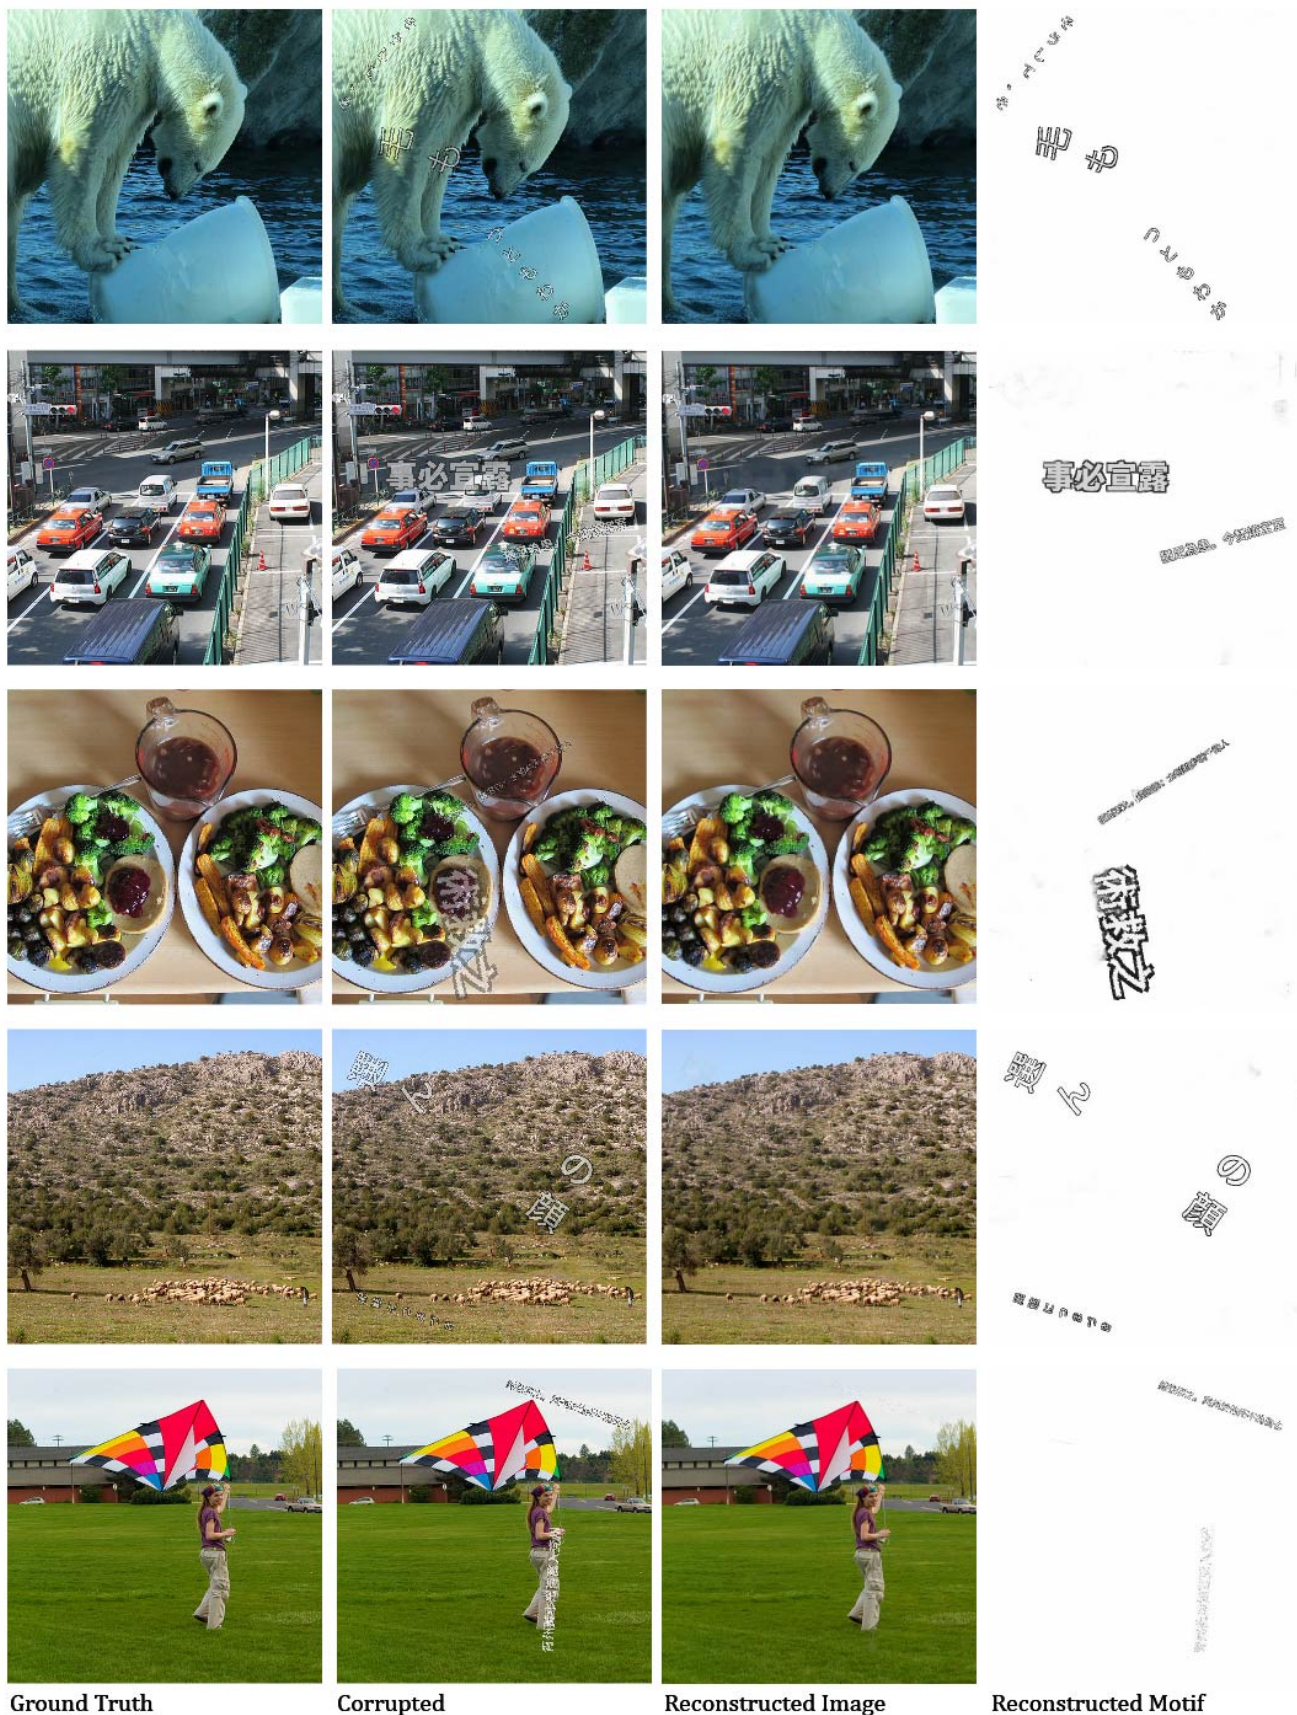

Figure 7: Examples of semi-transparent visual motif removal results. The test images contains unseen images and unseen characters as the visual motif.

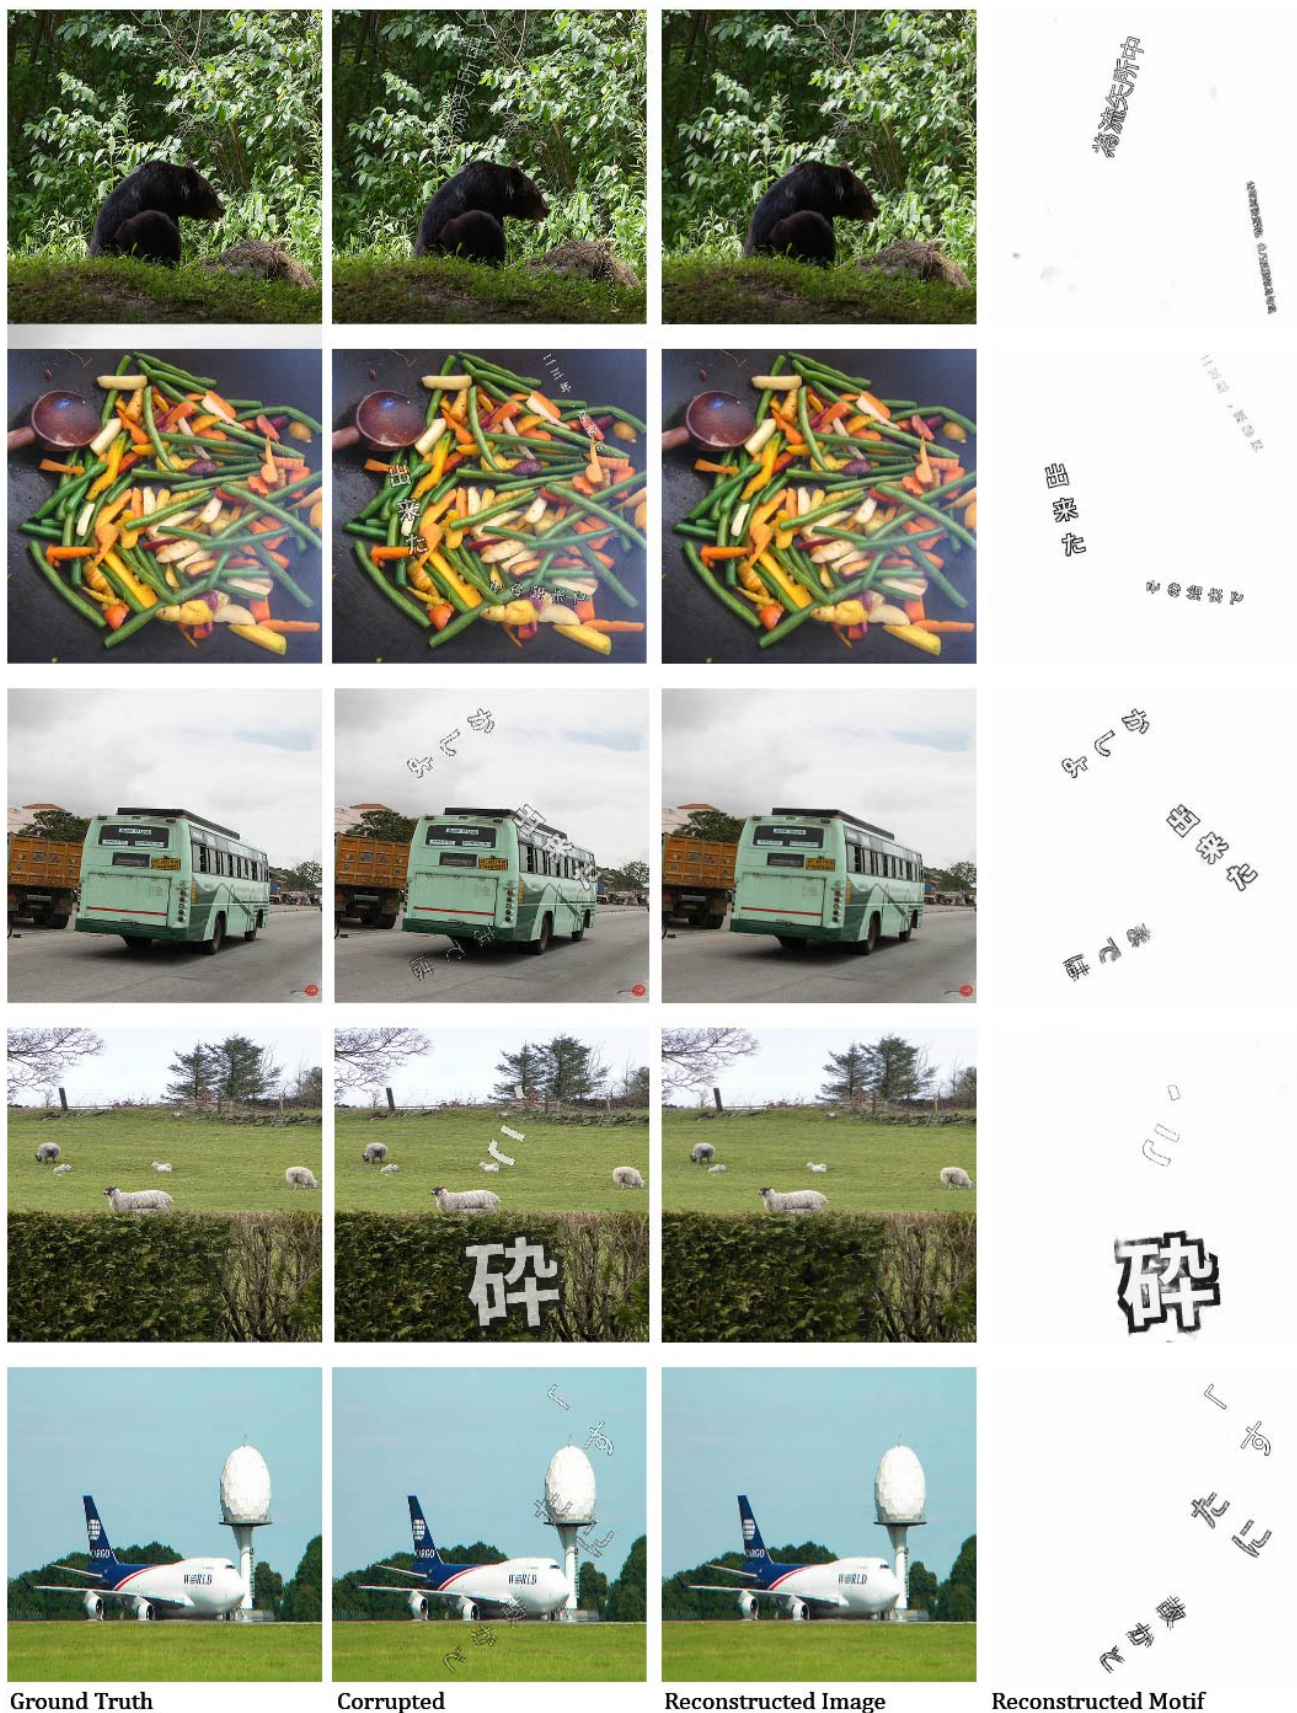

Figure 8: Examples of semi-transparent visual motif removal results. The test images contains unseen images and unseen characters as the visual motif.

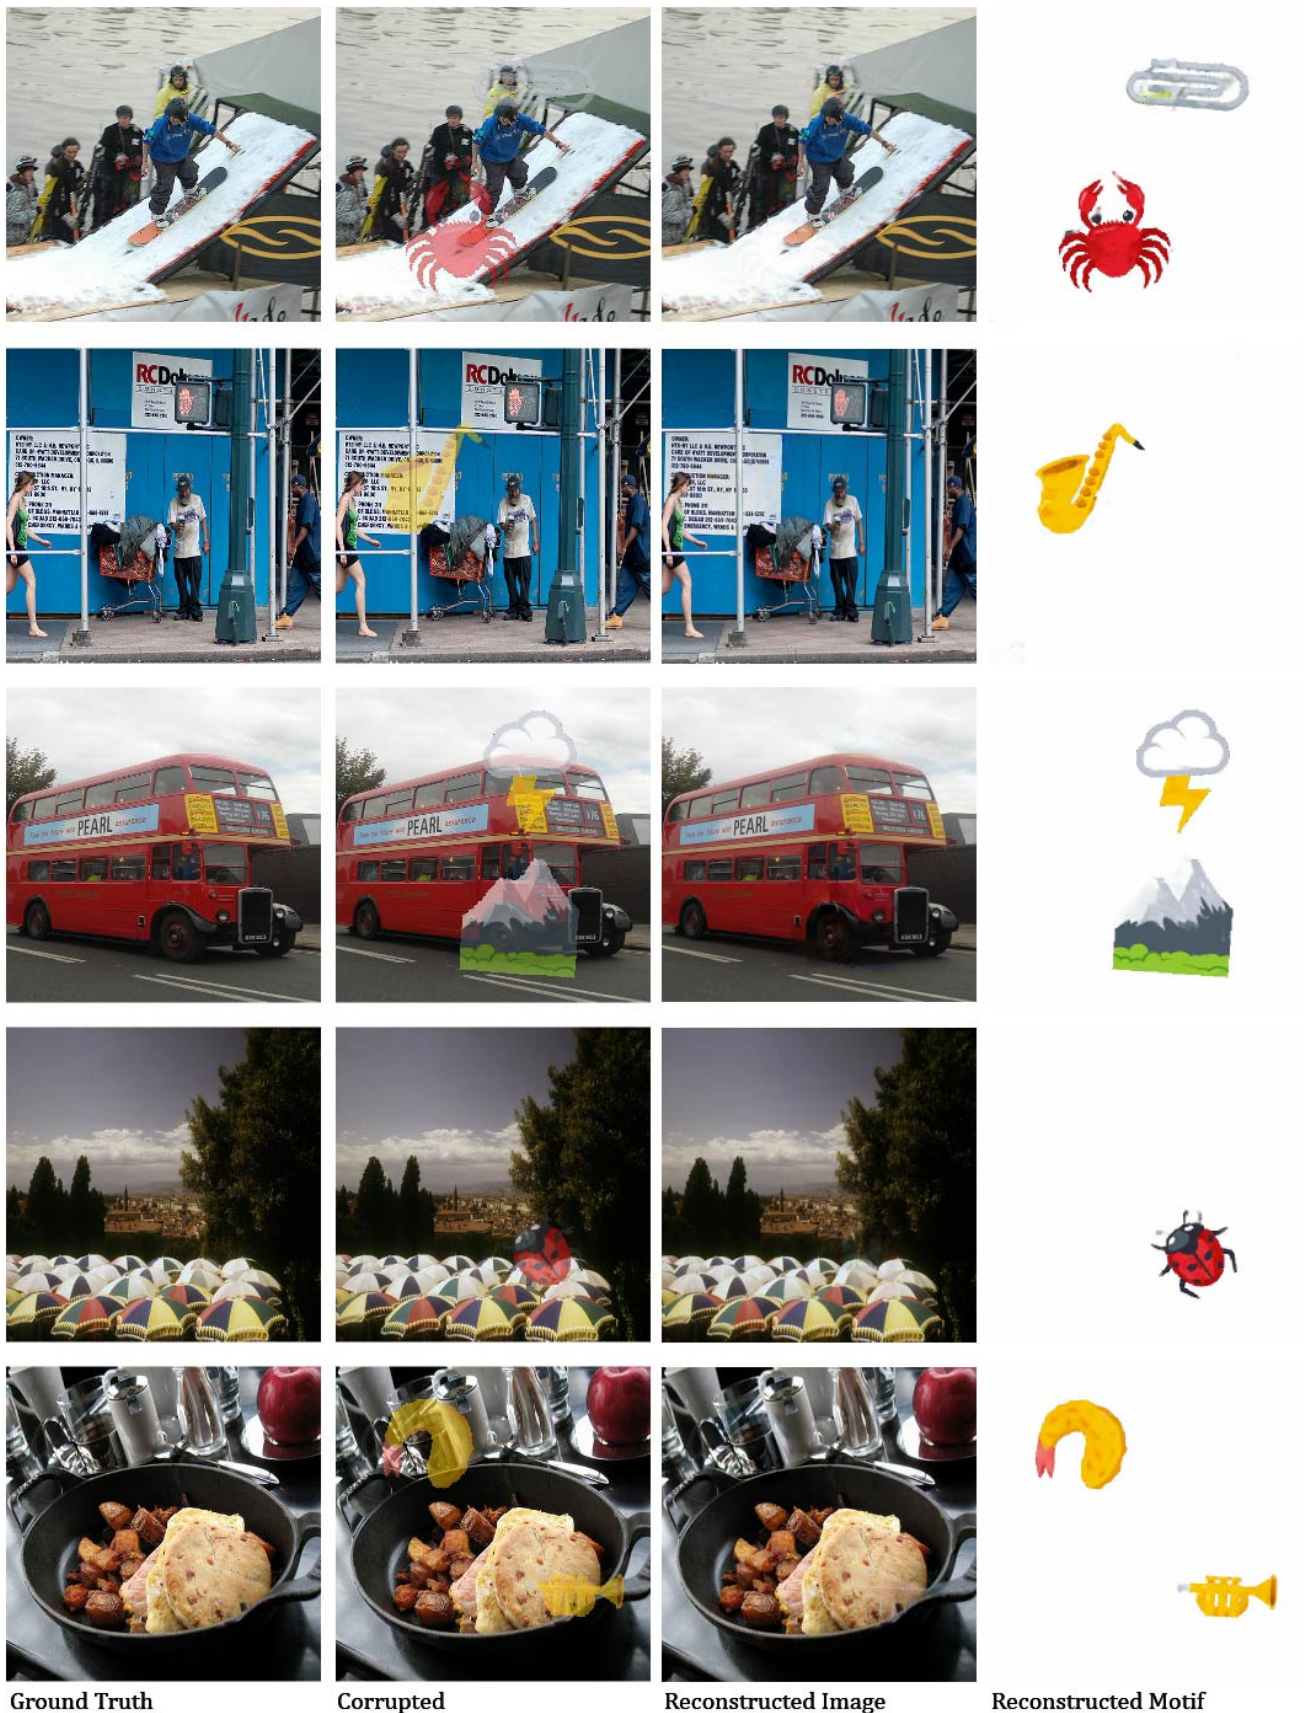

Figure 9: Examples of semi-transparent visual motif removal results. The test images contains unseen images and unseen emojis as the visual motif.

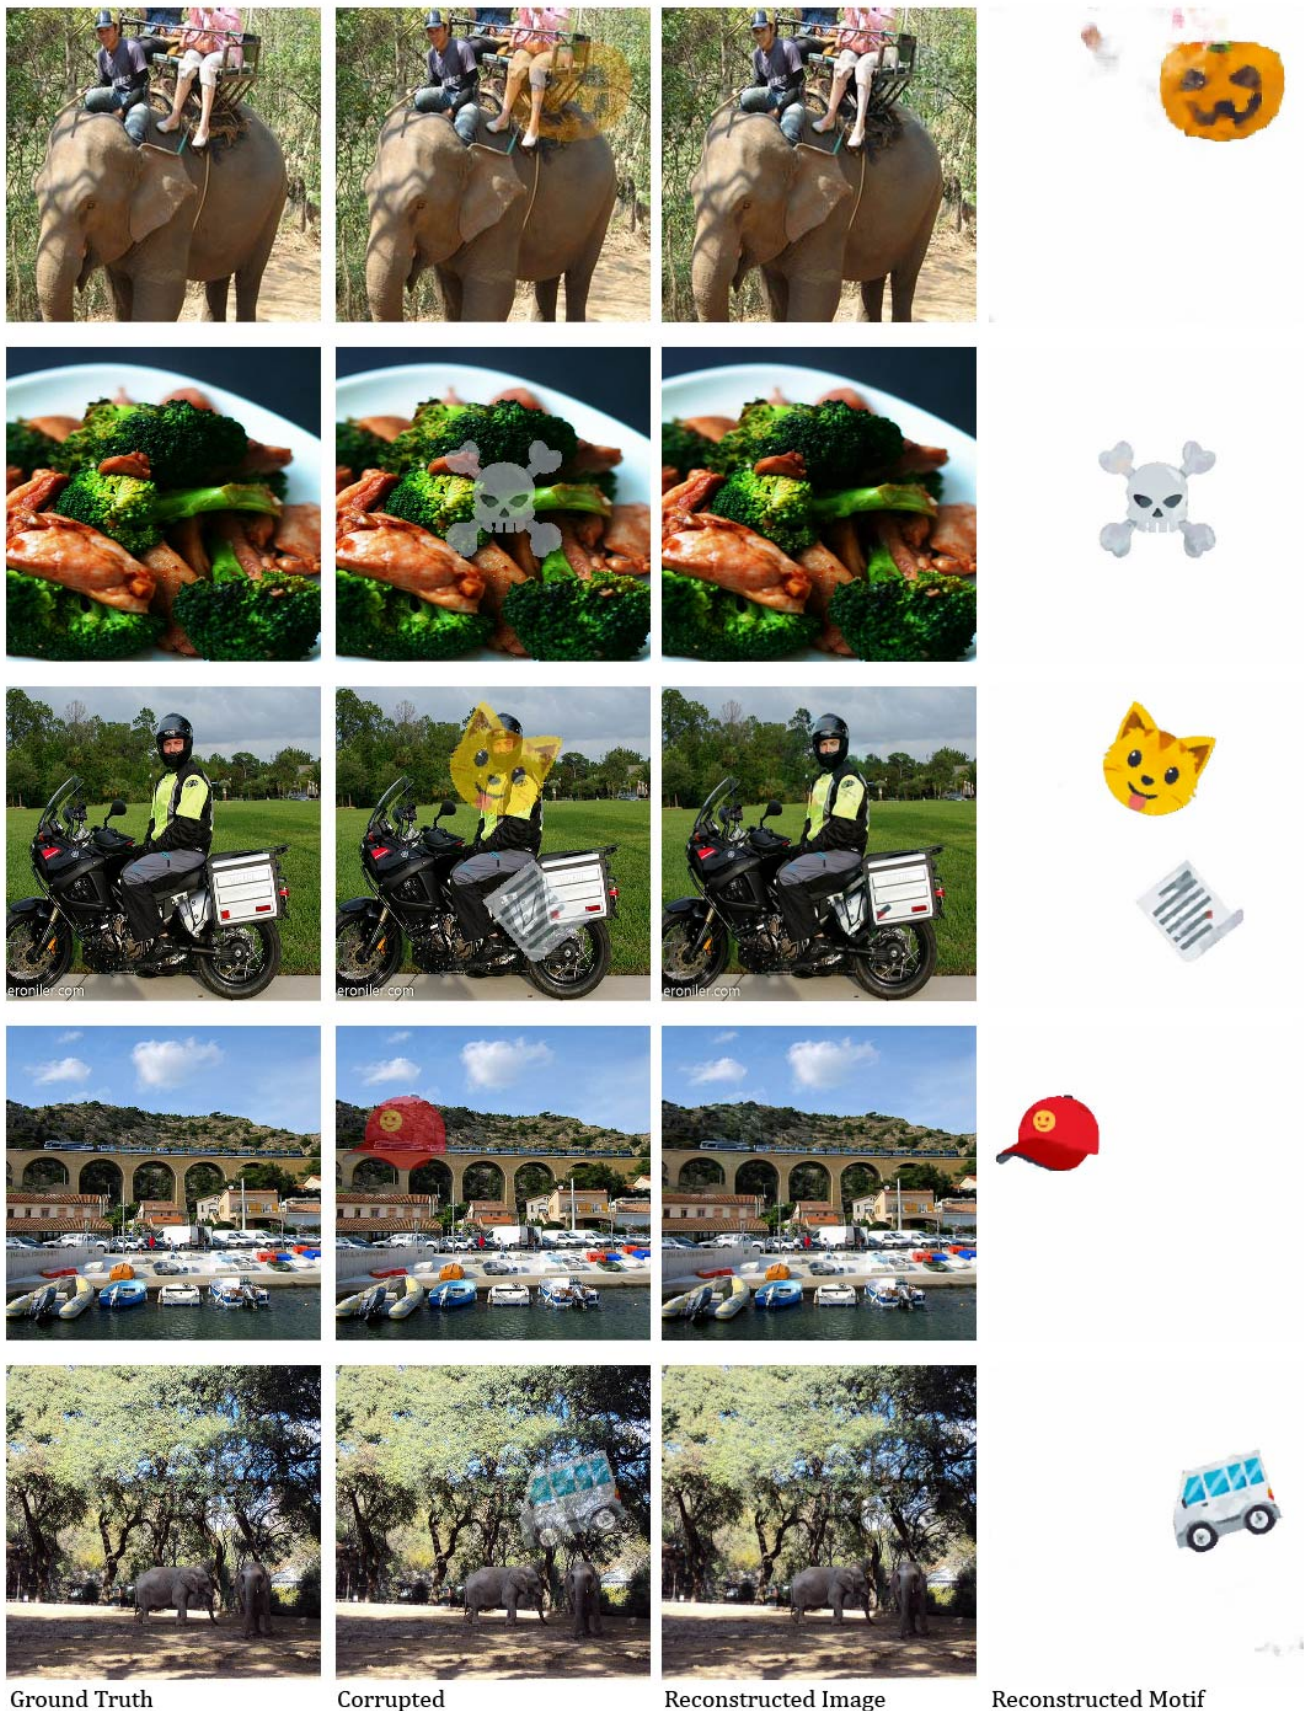

Figure 10: Examples of semi-transparent visual motif removal results. The test images contains unseen images and unseen emojis as the visual motif.

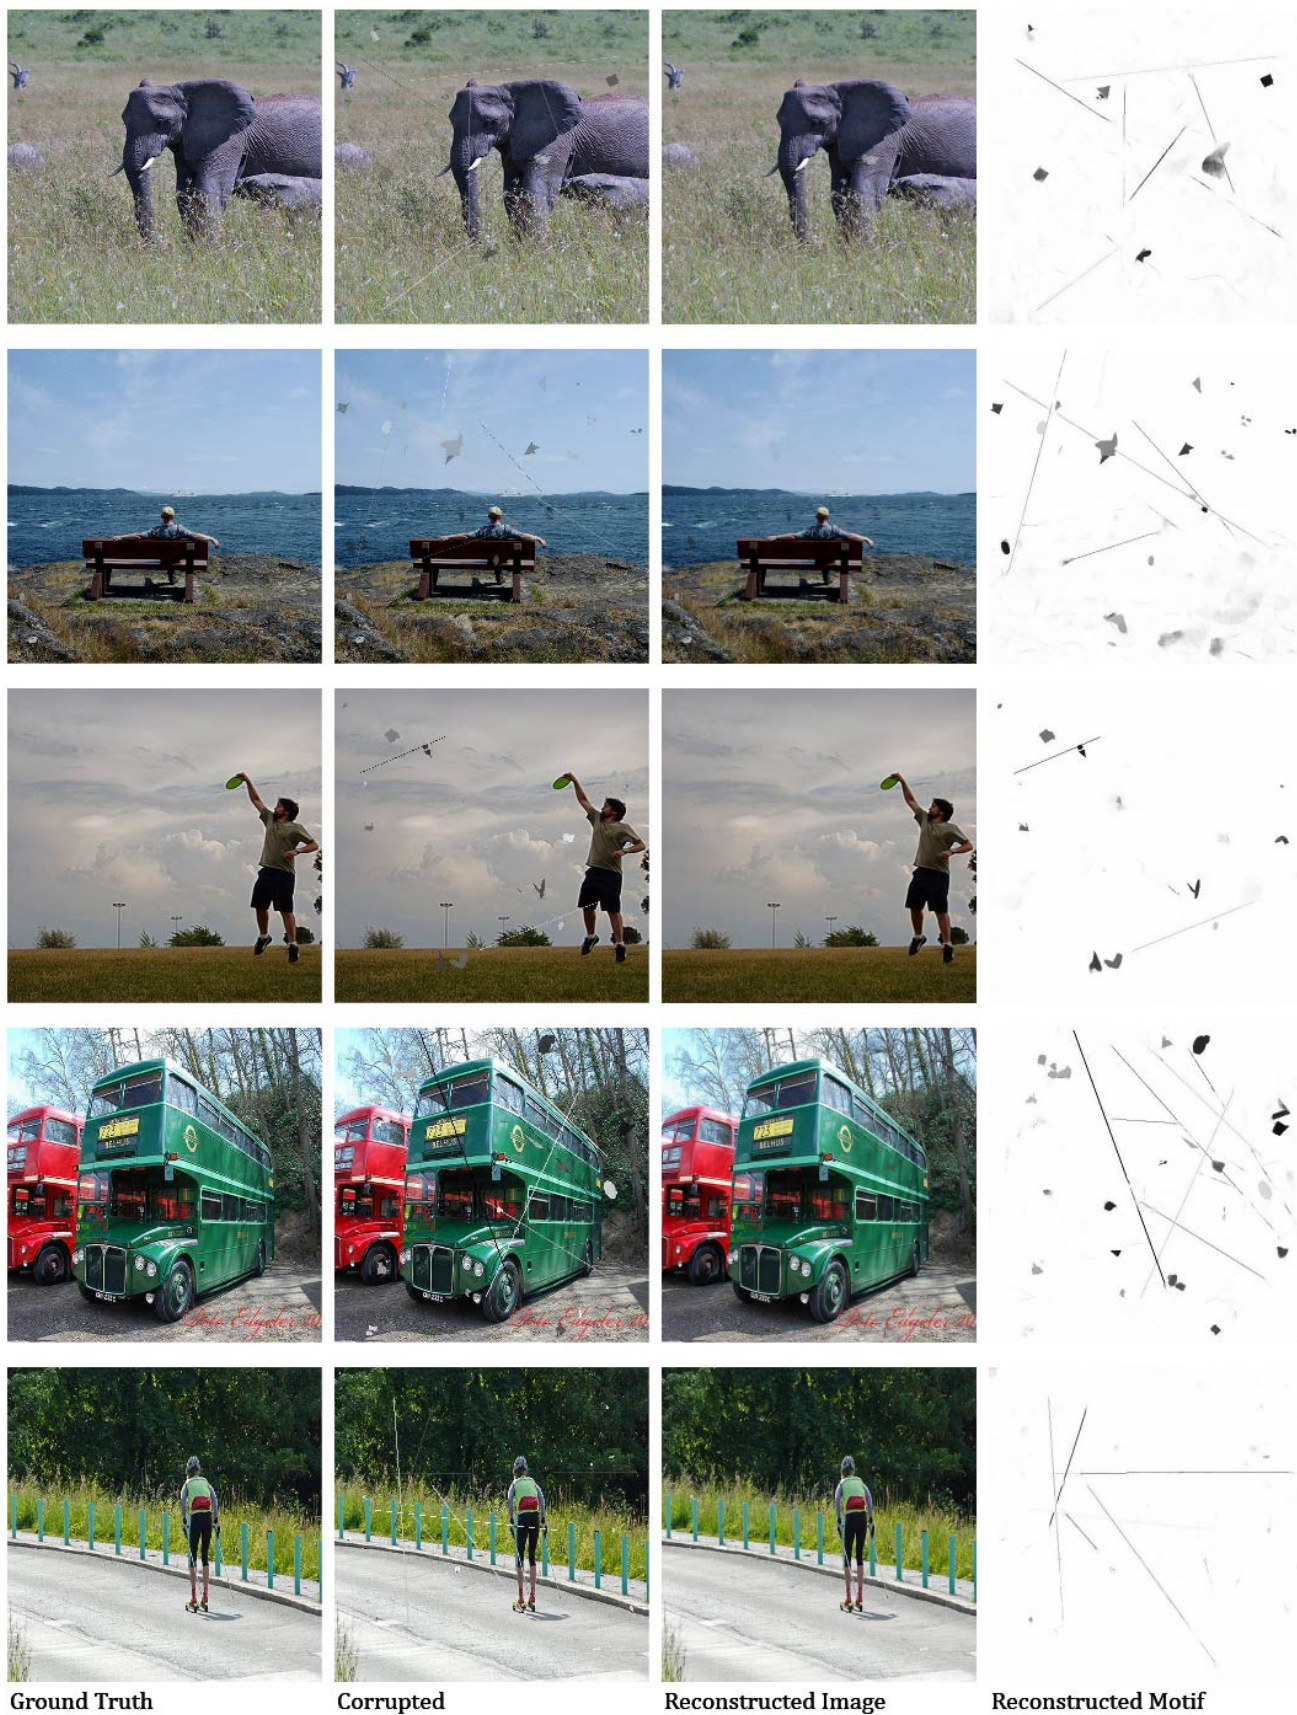

Figure 11: Examples of semi-transparent visual motif removal results on geometric shapes as the visual motif.

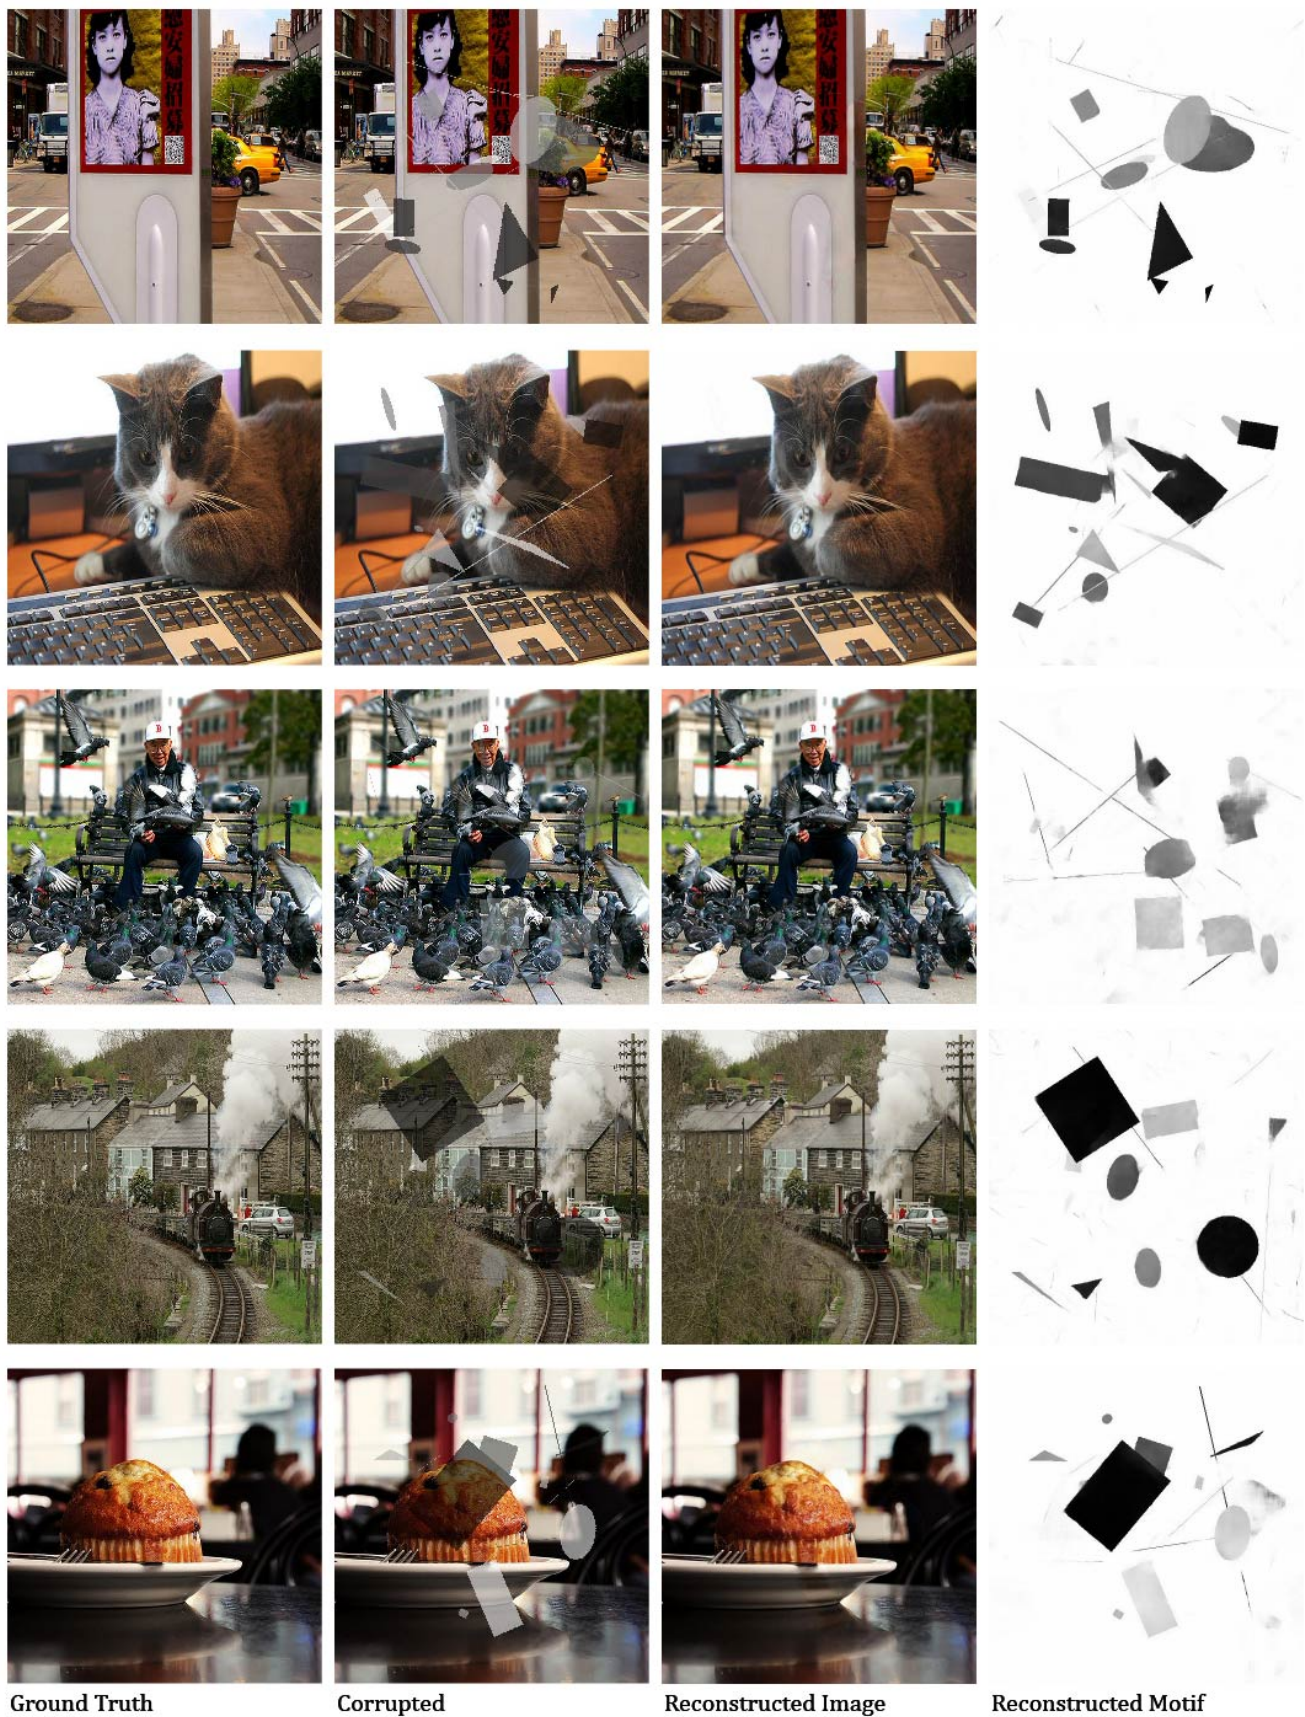

Figure 12: Examples of semi-transparent visual motif removal results on geometric shapes as the visual motif.

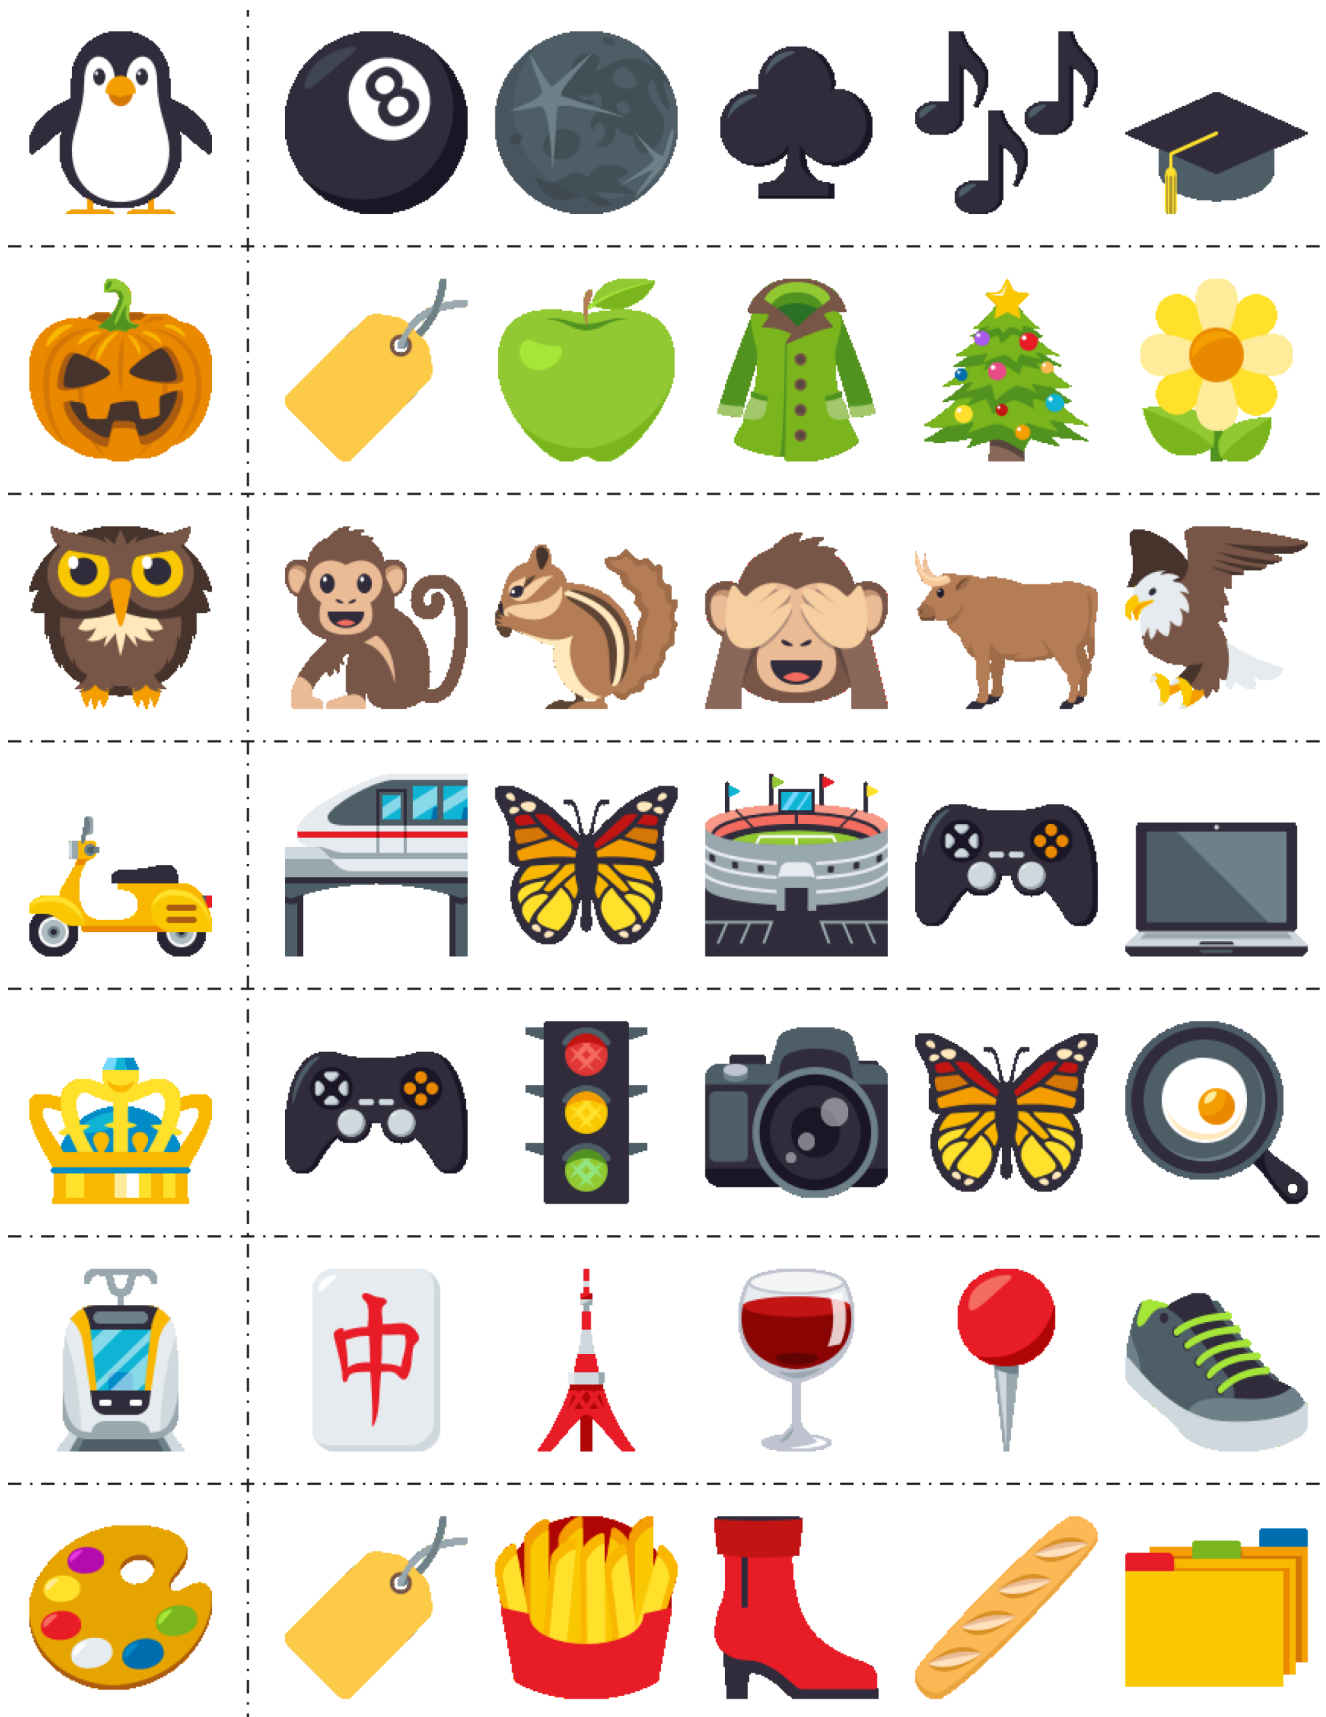

Figure 13: Examples of emojis removed during test time and their five nearest neighbors from the training dataset.

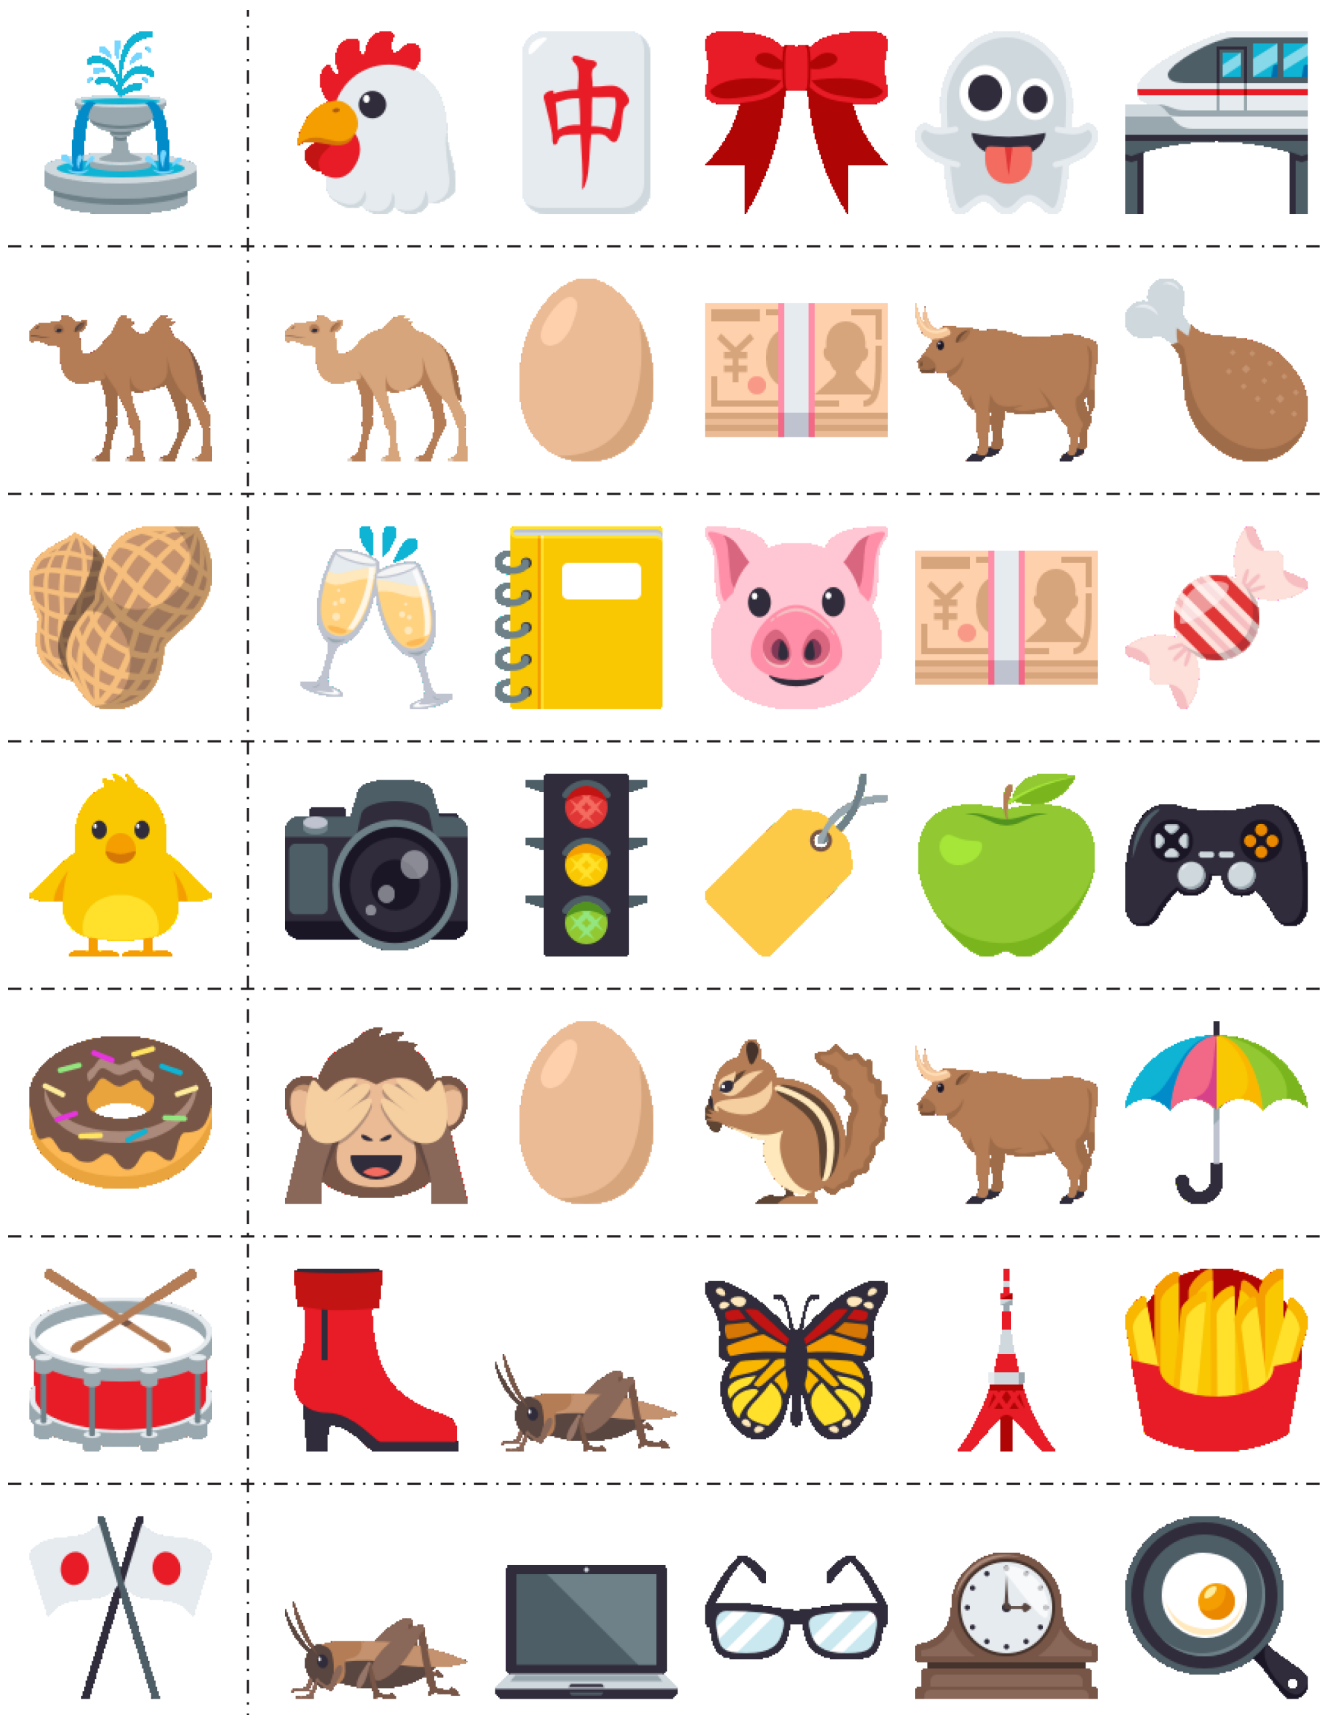

Figure 14: Examples of emojis removed during test time and their five nearest neighbors from the training dataset.

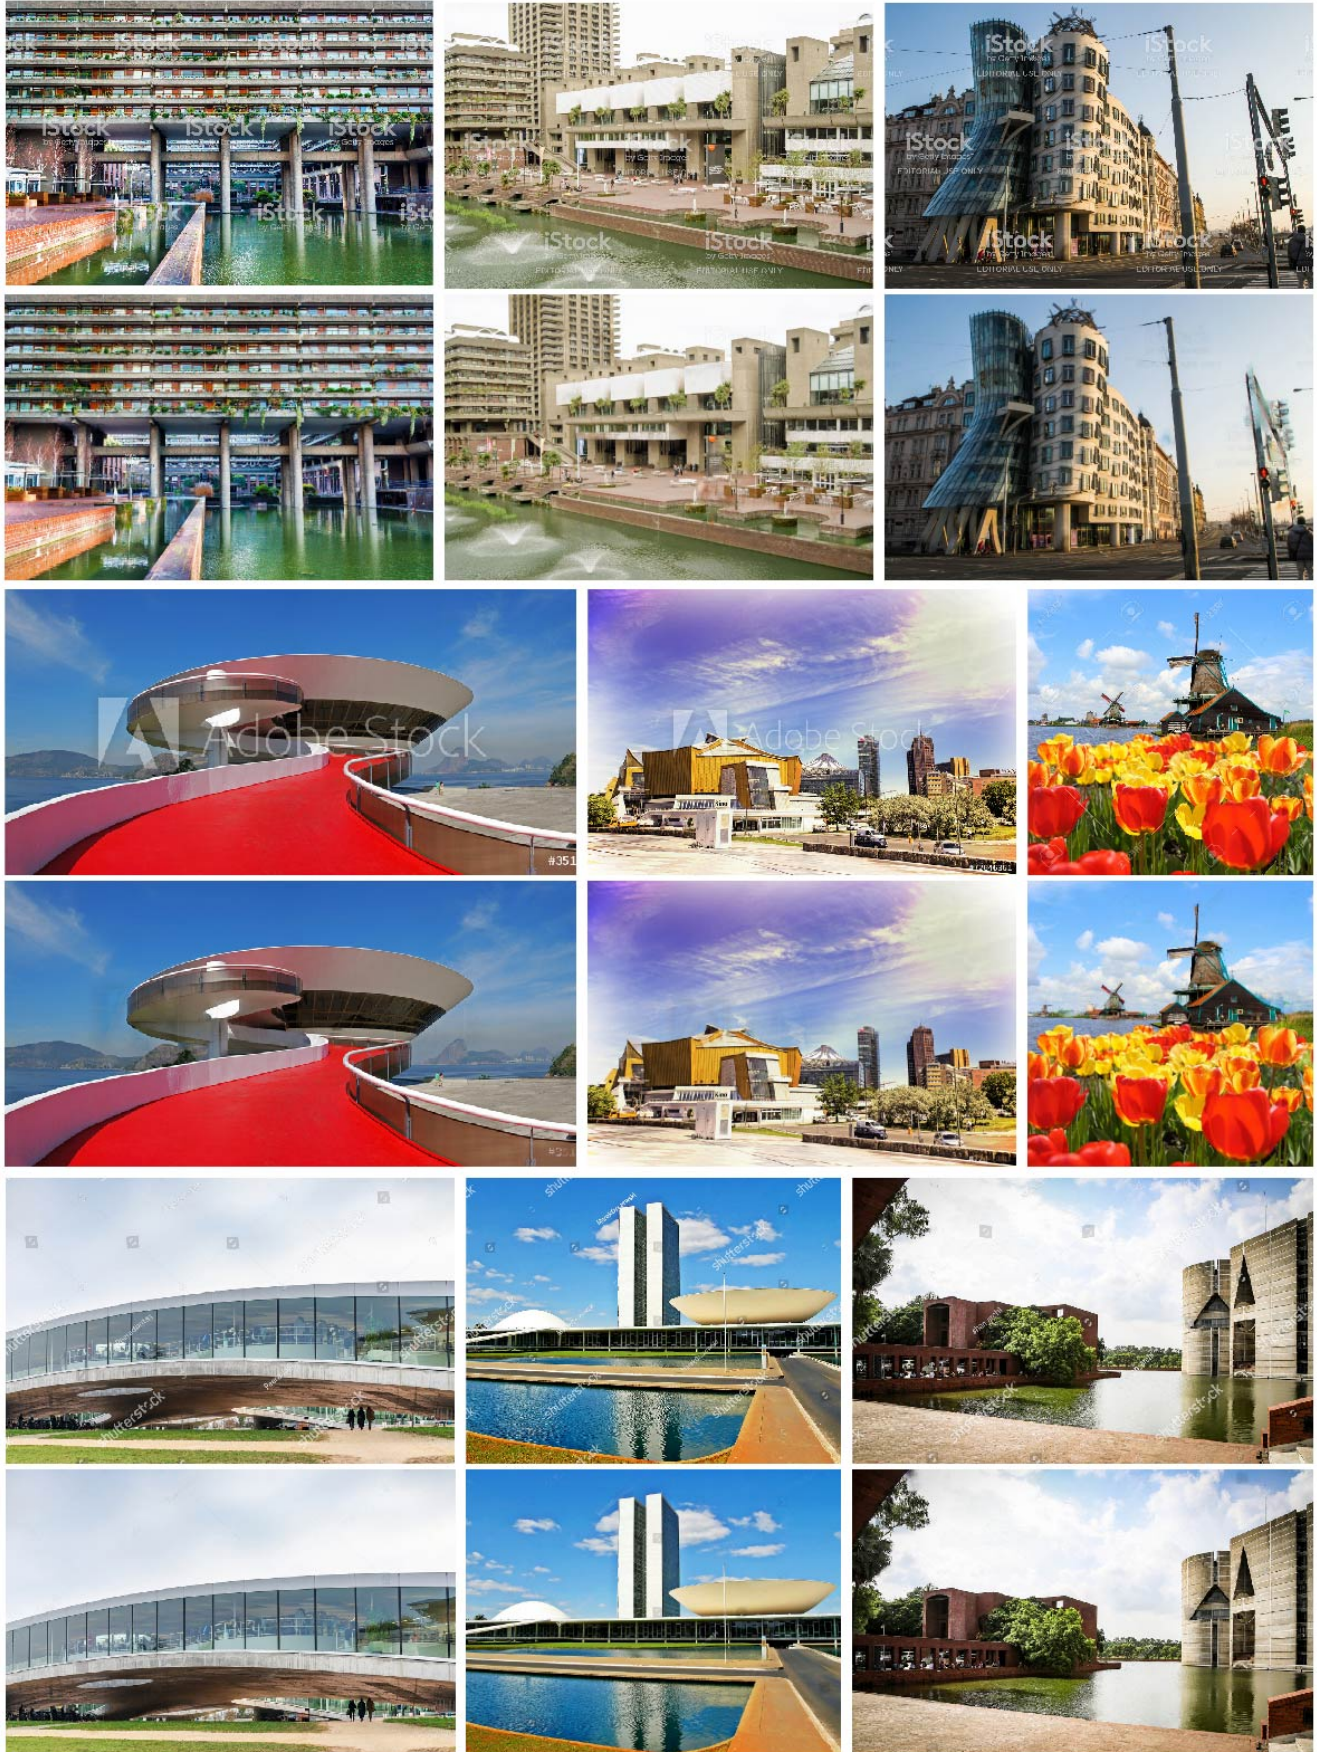

Figure 15: Watermark removal examples on stock imagery downloaded from *AdobeStock*, *123RF*, *Shutterstock* and *iStock*. Our results are shown beneath each image.

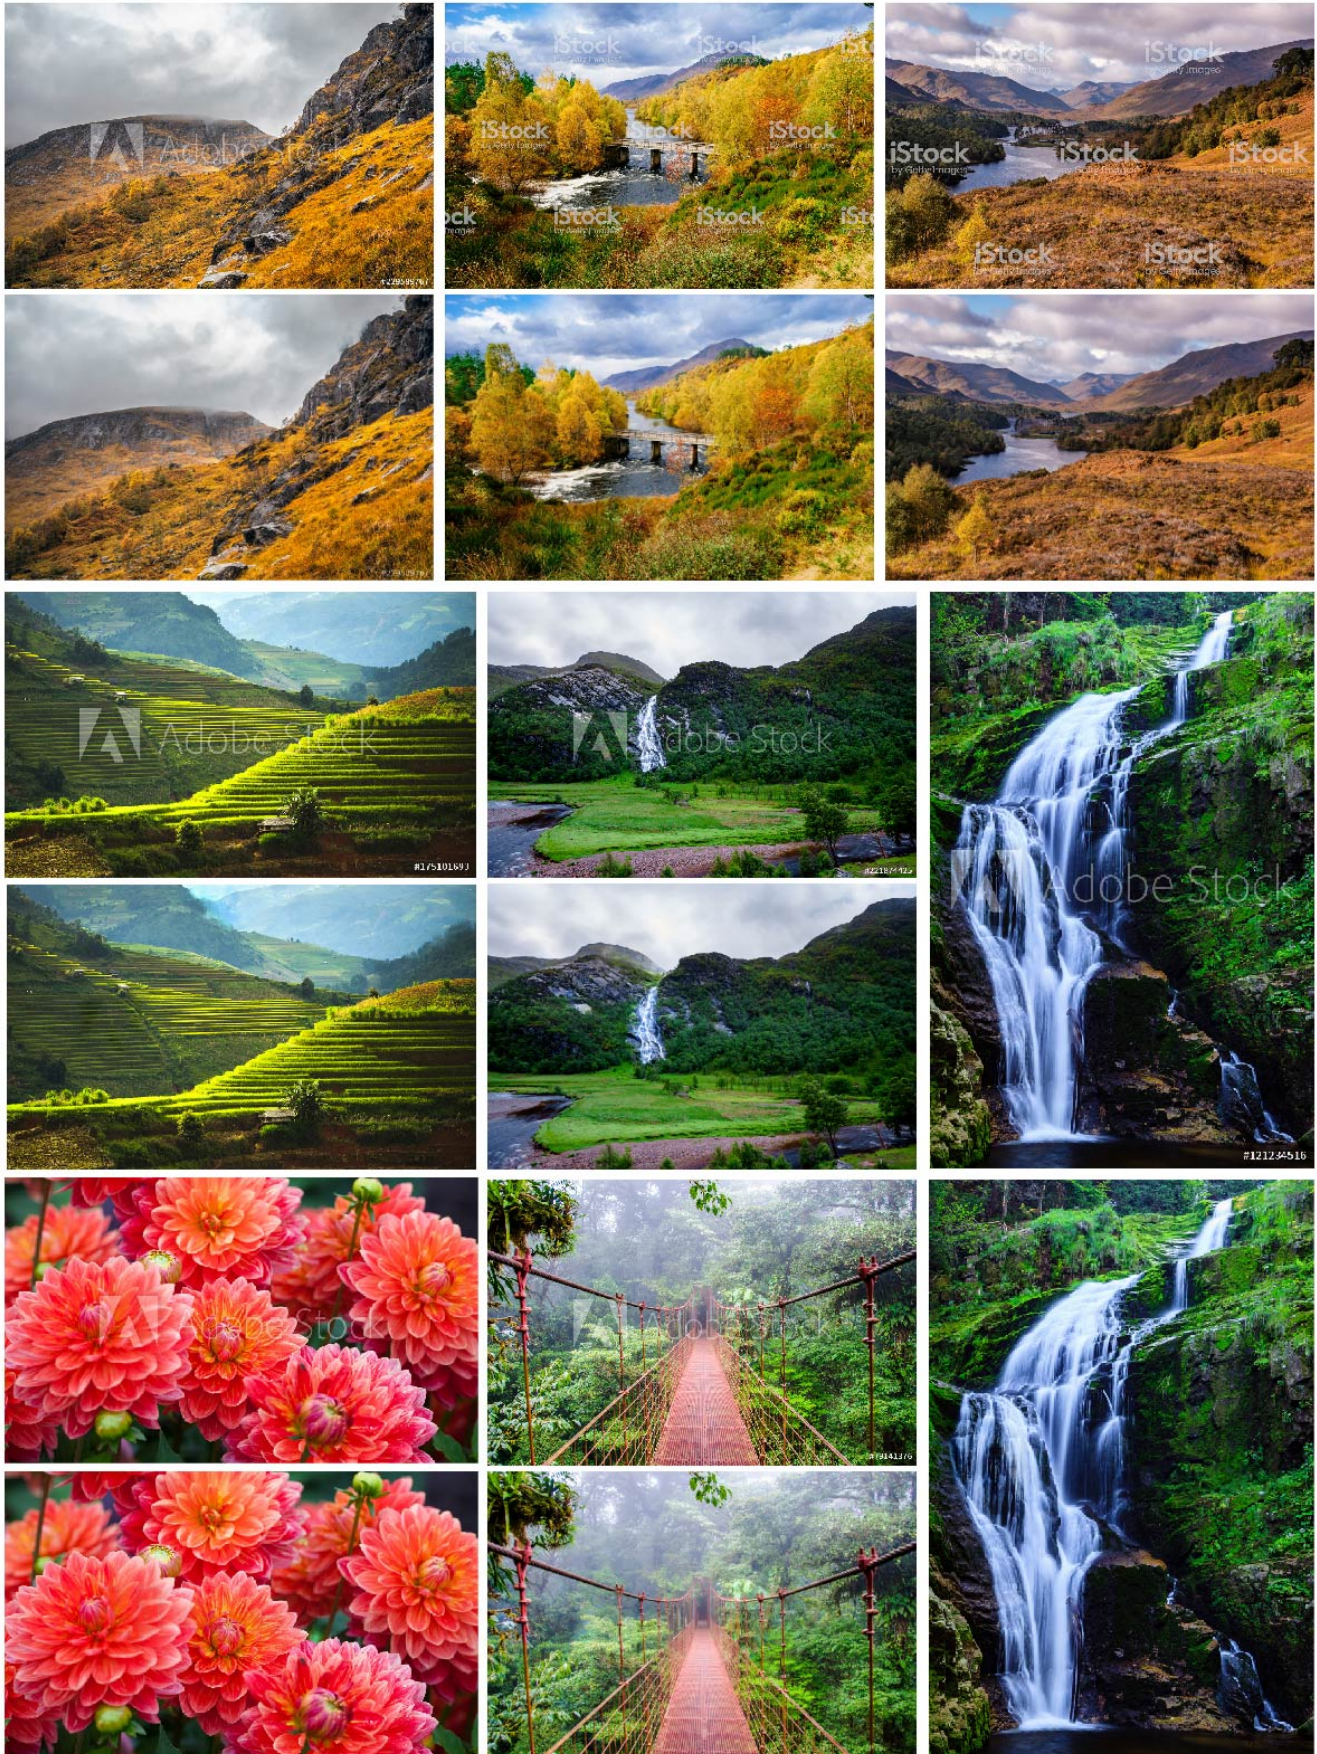

Figure 16: Watermark removal examples on stock imagery downloaded from *AdobeStock*, *123RF*, *Shutterstock* and *iStock*. Our results are shown beneath each image.

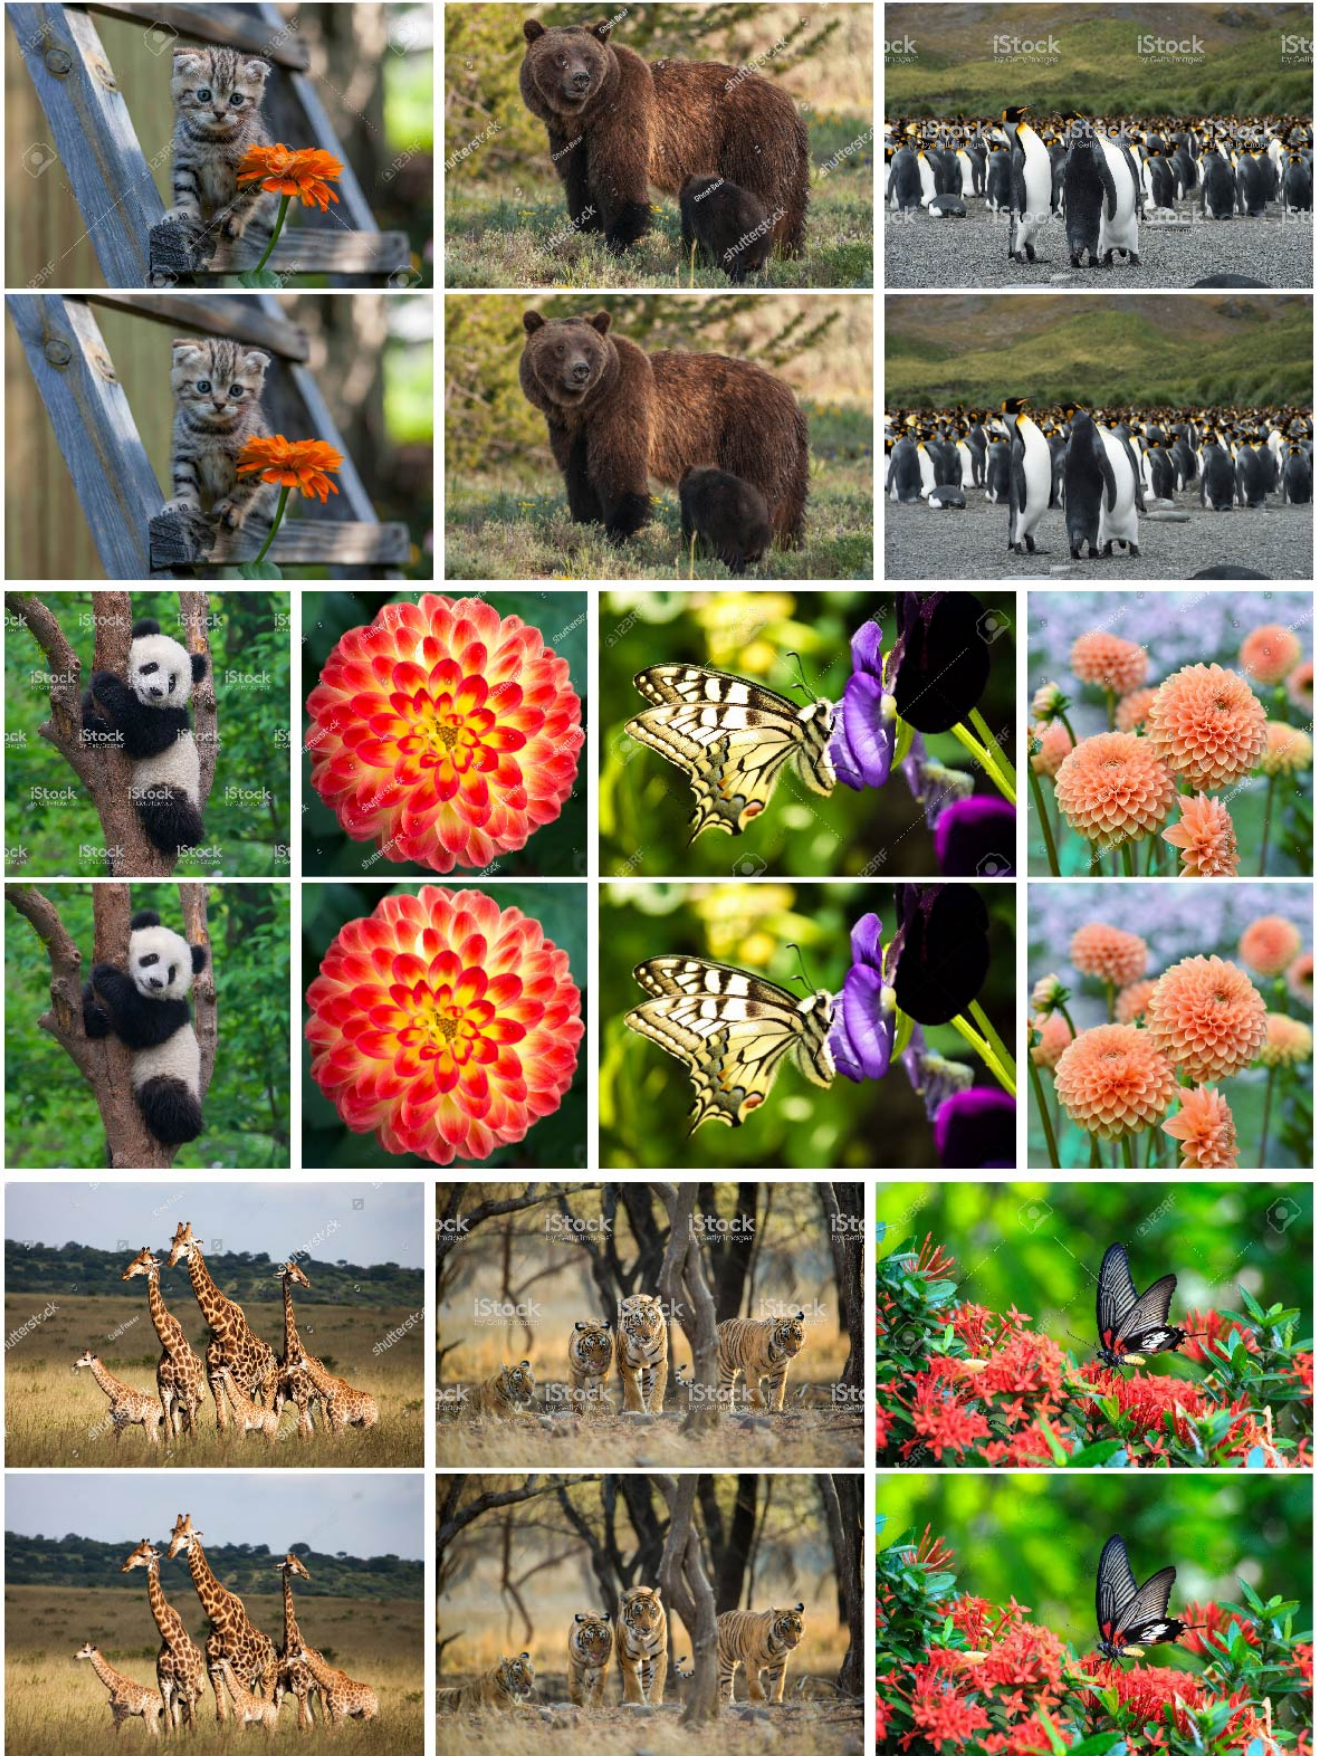

Figure 17: Watermark removal examples on stock imagery downloaded from *AdobeStock*, *123RF*, *Shutterstock* and *iStock*. Our results are shown beneath each image.

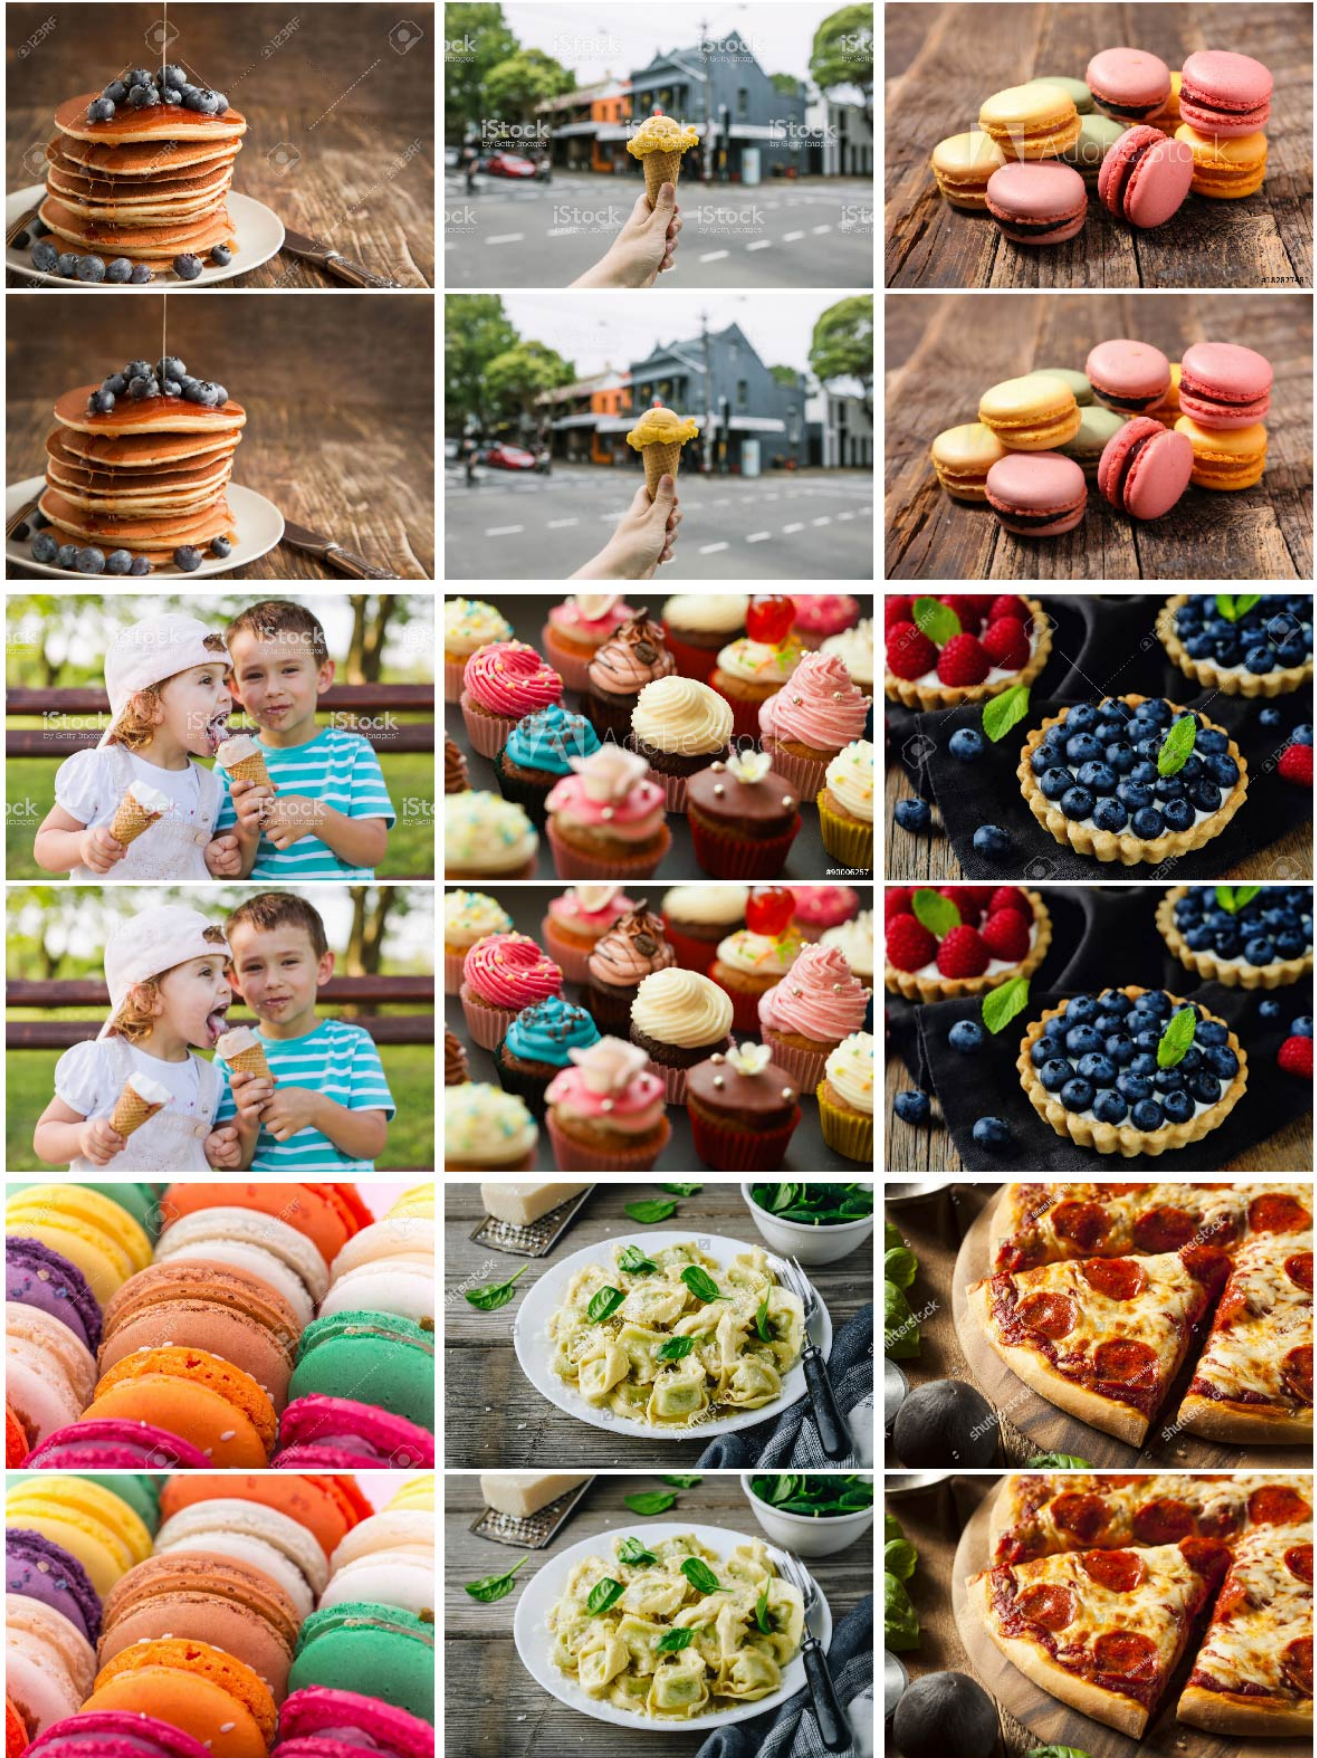

Figure 18: Watermark removal examples on stock imagery downloaded from *AdobeStock*, *123RF*, *Shutterstock* and *iStock*. Our results are shown beneath each image.

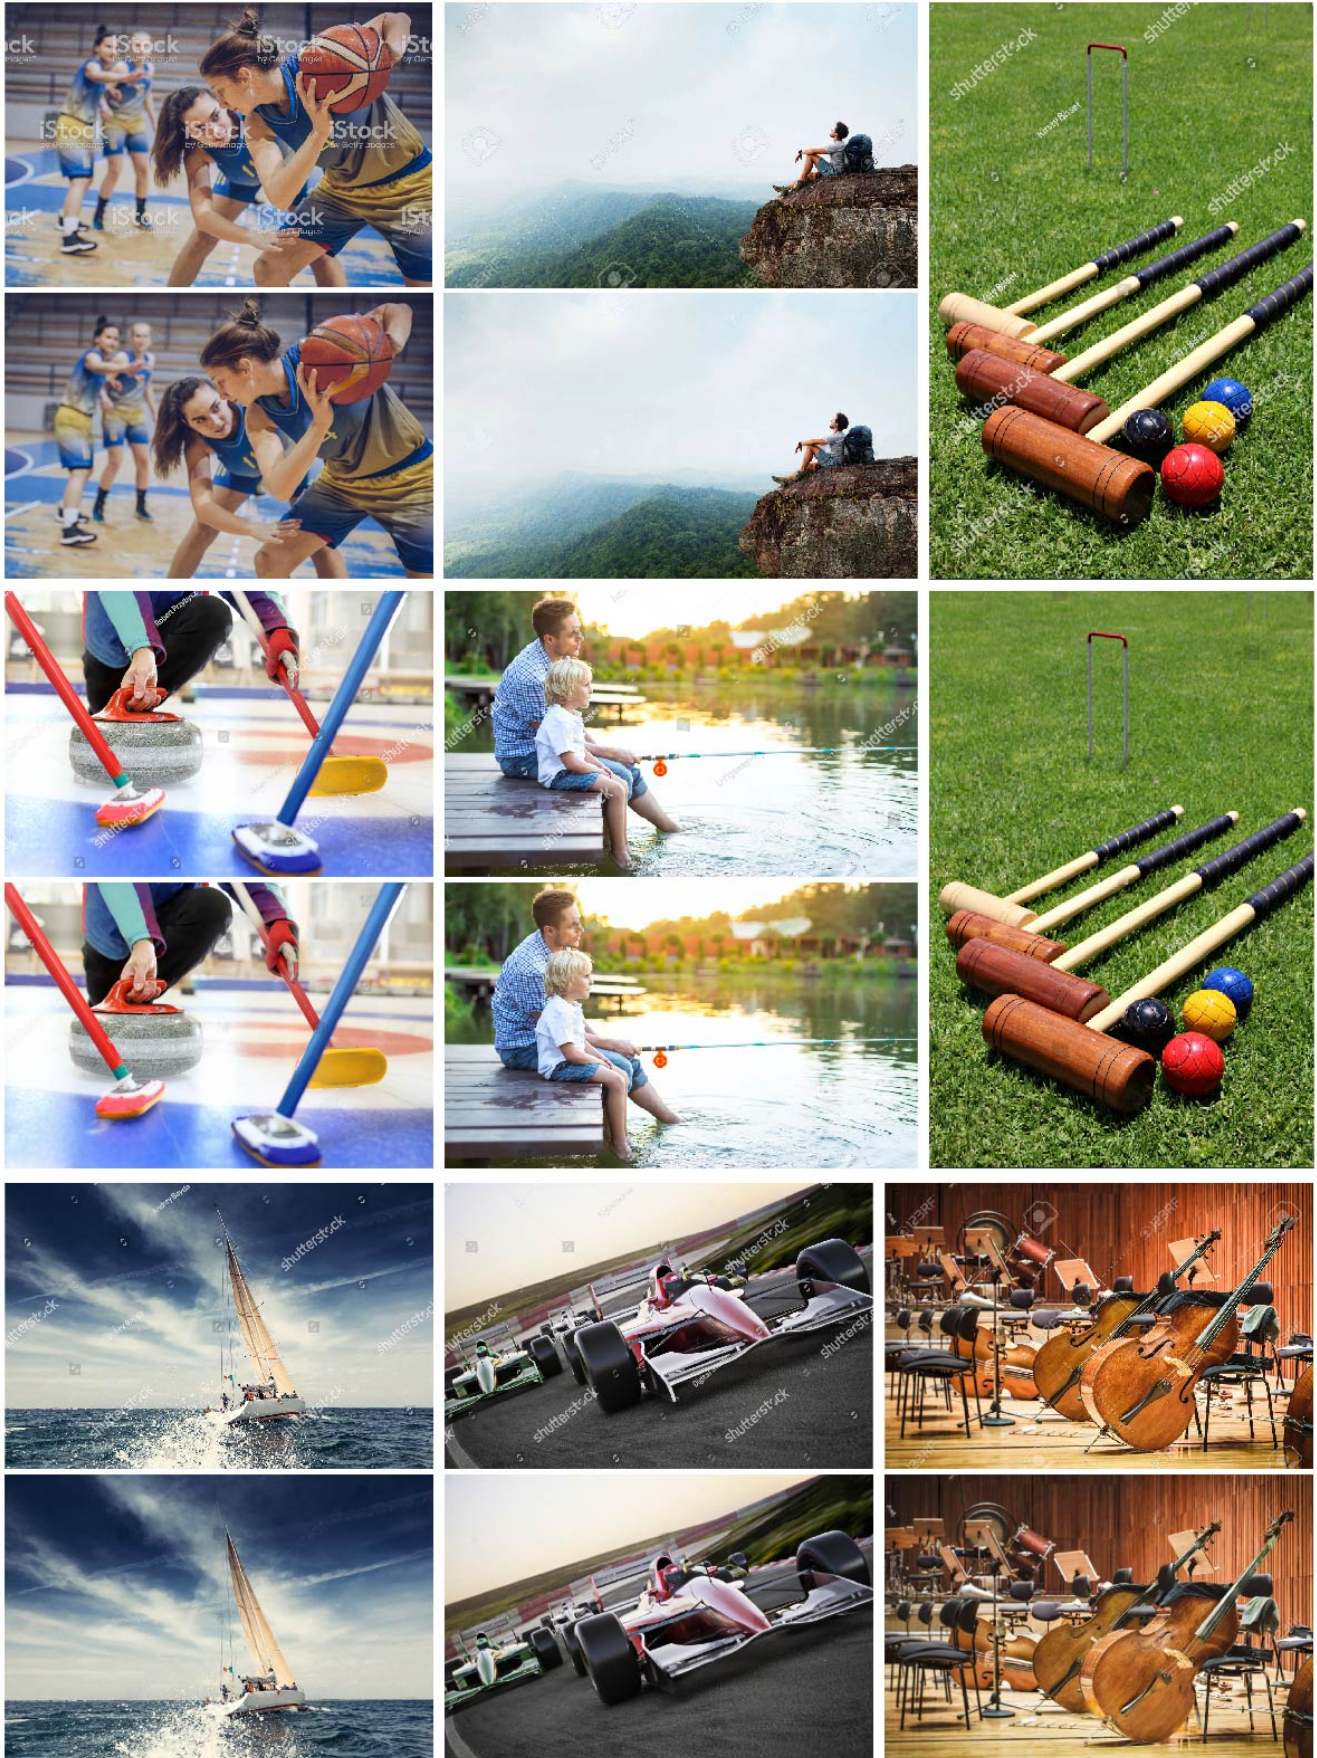

Figure 19: Watermark removal examples on stock imagery downloaded from *AdobeStock*, *123RF*, *Shutterstock* and *iStock*. Our results are shown beneath each image.

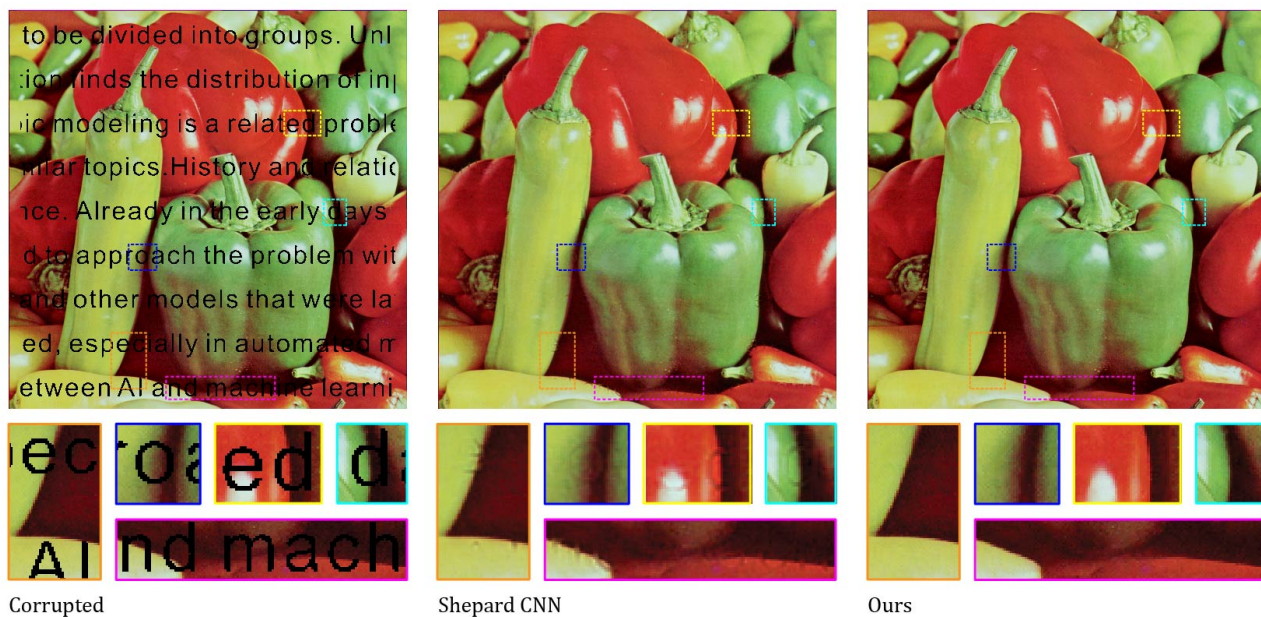

Figure 20: Visual comparison on Shepard-CNN sample photo [5].

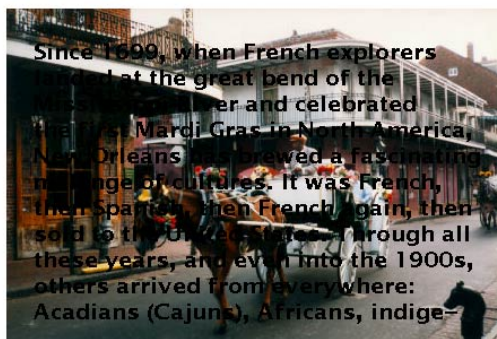

Corrupted

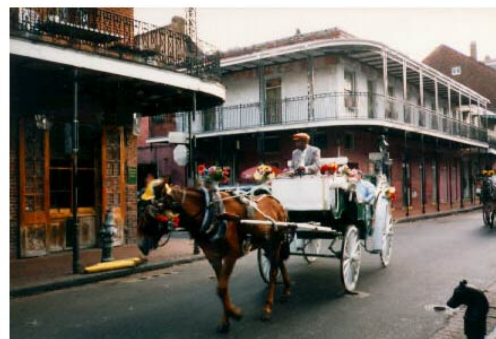

FoE

31.668 / 0.972

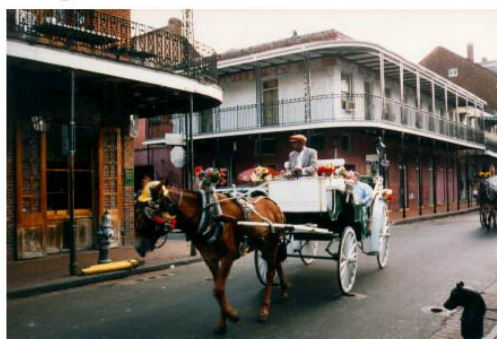

Ground Truth

PSNR / SSIM

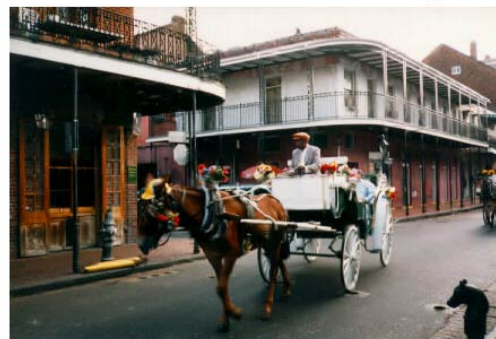

EPLL

32.665 / 0.972

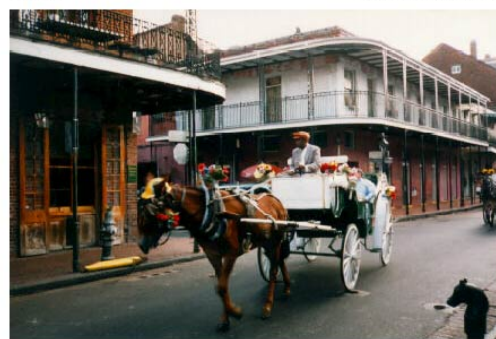

Ours

33.095 / 0.976

Figure 21: Comparison with EPLL [6] and FoE [7] on their sample image.

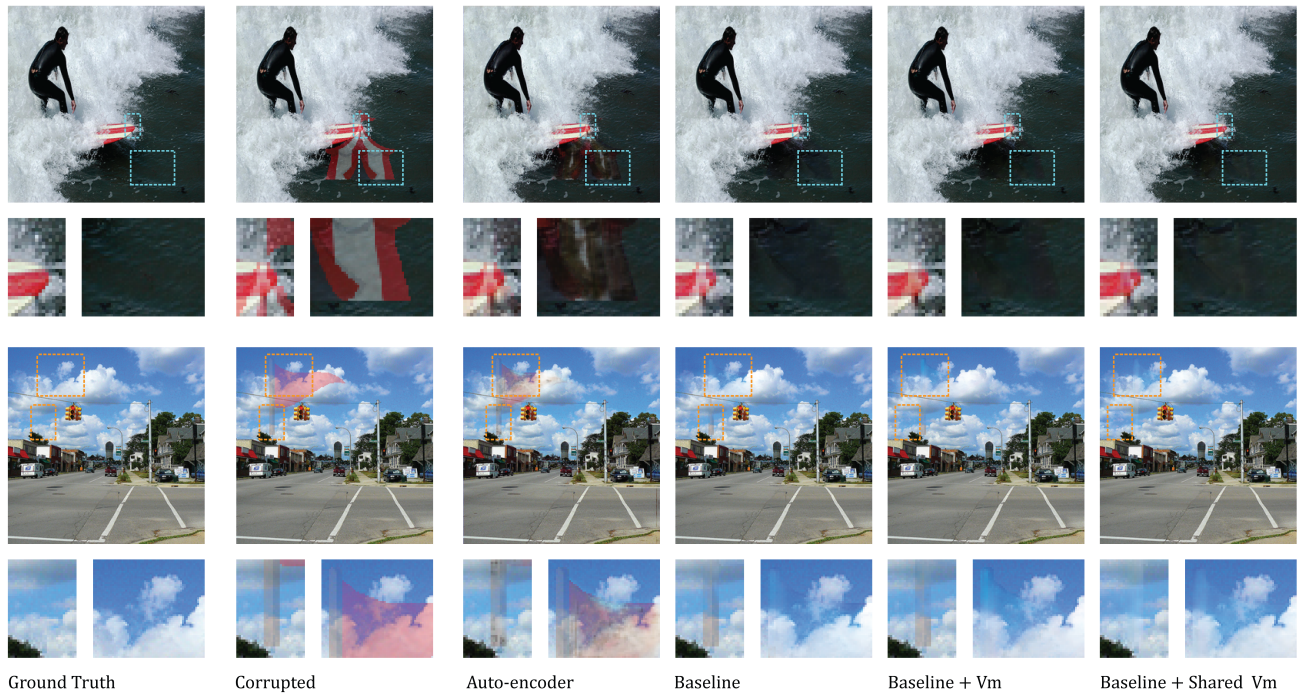

Figure 22: Ablation study: A qualitative evaluation of the different architectures. As the images show, using a network that identifies the pixels with the visual motif compared to using only a reconstruction loss improves the results greatly. Adding a third decoder to reconstruct the visual motif and sharing the weights between the two reconstructing decoders leads to even better results.
